# Supplementary material for: Optimizing Cross-Domain Transfer for Universal Machine Learning Interatomic Potentials
Source: arXiv:2510.11241 ancillary file (2025-11-07)
Supplement: Supplementary file 1 [file si.pdf]

# Supplementary information: Optimizing Cross-Domain Transfer for Universal Machine Learning Interatomic Potentials

Jaesun Kim[1†], Jinmu You[1†], Yutack Park[1], Yunsung Lim[2], Yujin Kang[1], Jisu Kim[1], Haekwan Jeon[1], Suyeon Ju[1], Deokgi Hong[1], Seung Yul Lee[3], Saerom Choi[1,4], Yongdeok Kim[4], Jae W. Lee[3], Seungwu Han[1,2,5*]

[1]Department of Materials Science and Engineering, Seoul National University, Seoul, 08826, Republic of Korea.

[2]Research Institute of Advanced Materials, Seoul National University, Seoul, 08826, Republic of Korea.

[3]Department of Computer Science and Engineering, Seoul National University, Seoul, 08826, Republic of Korea.

[4]AI Center, Samsung Electronics, Suwon, 16678, Republic of Korea.

[5]Center for AI and Natural Sciences, Korea Institute of Advanced Study, Seoul, 02455, Republic of Korea.

*Corresponding author(s). E-mail(s): hansw@snu.ac.kr;

†These authors contributed equally to this work.

**Supplementary Table 1**: Composition of the domain-bridging database. The fraction represents the sampling ratio relative to the original database.

| Database | Number of samples | Fraction (%) |
|---|---:|---:|
| MatPES | 300 | 0.07 |
| OC20 | 18,000 | 0.06 |
| OC22 | 4,500 | 0.05 |
| ODAC23 | 2,400 | 0.06 |
| OMOL25 | 74,100 | 0.12 |
| QCML | 25,200 | 0.14 |

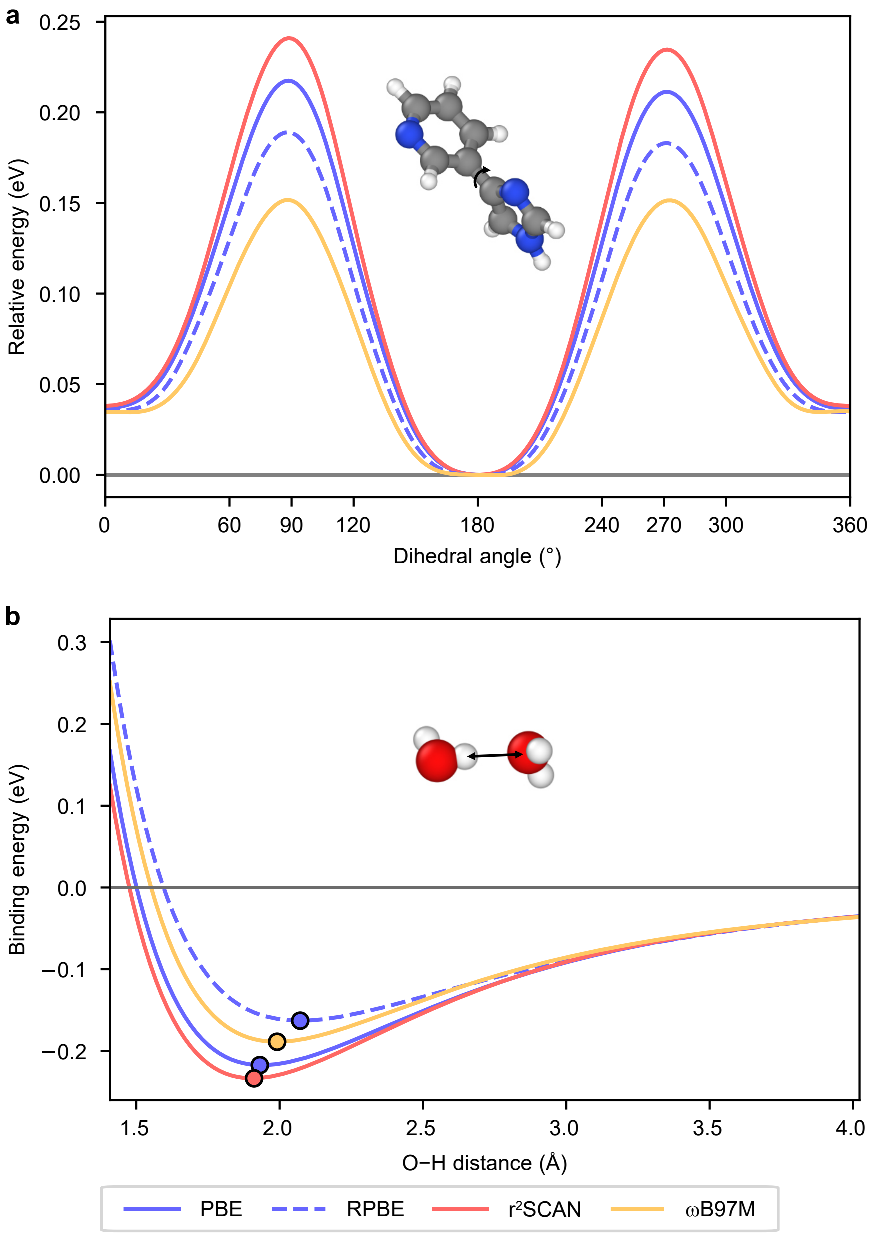


**Supplementary Figure 1**: **Potential energy surfaces of molecular systems with varying ab initio method.** Blue lines indicate PES obtained by GGA-type functionals, while red and yellow lines illustrate PES calculated with r$^2$SCAN and $\omega$B97M functional, respectively. Among blue lines, solid lines and dashed lines corresponds to PBE and RPBE PES. **a** Torsional PES obtained by rotating dihedral angle of a biaryl molecule. **b** Energy landscape of water molecule dimer by varying distance between the two. Circle markers indicate equilibrium distance with the lowest energy for each functional.

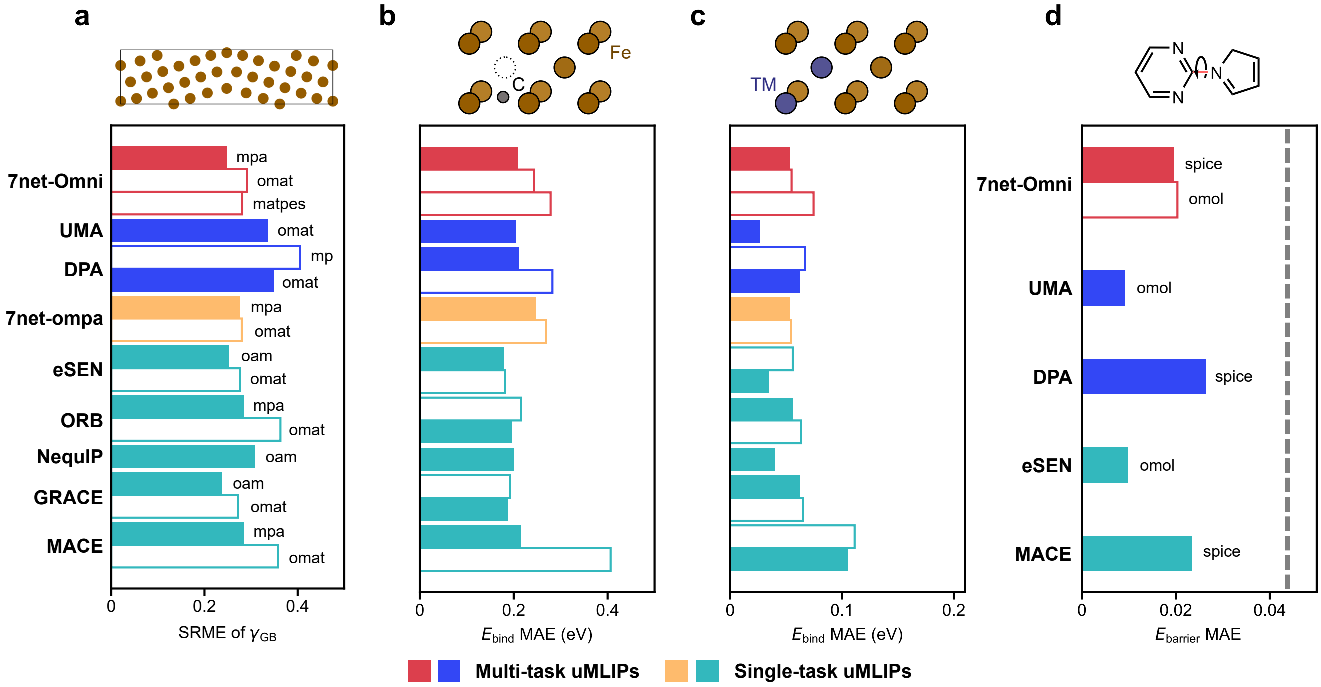


**Supplementary Figure 2**: **Performance of uMLIPs in single-domain tasks. a** SRME of grain boundary energies of elemental metals. **b** MAE of binding energies between carbon interstitials and vacancies in steels. **c** MAE of binding energies between transition metal solutes in steels. **d** MAE of torsional barriers. Gray dashed line denotes the error of 1 kcal/mol. Reference DFT data are calculated at the (**a**,**b**,**c**) PBE and (**d**) $\omega$B97M-D3 levels of theory. Individual parity plots are presented in Supplementary Fig. 3 to 6.

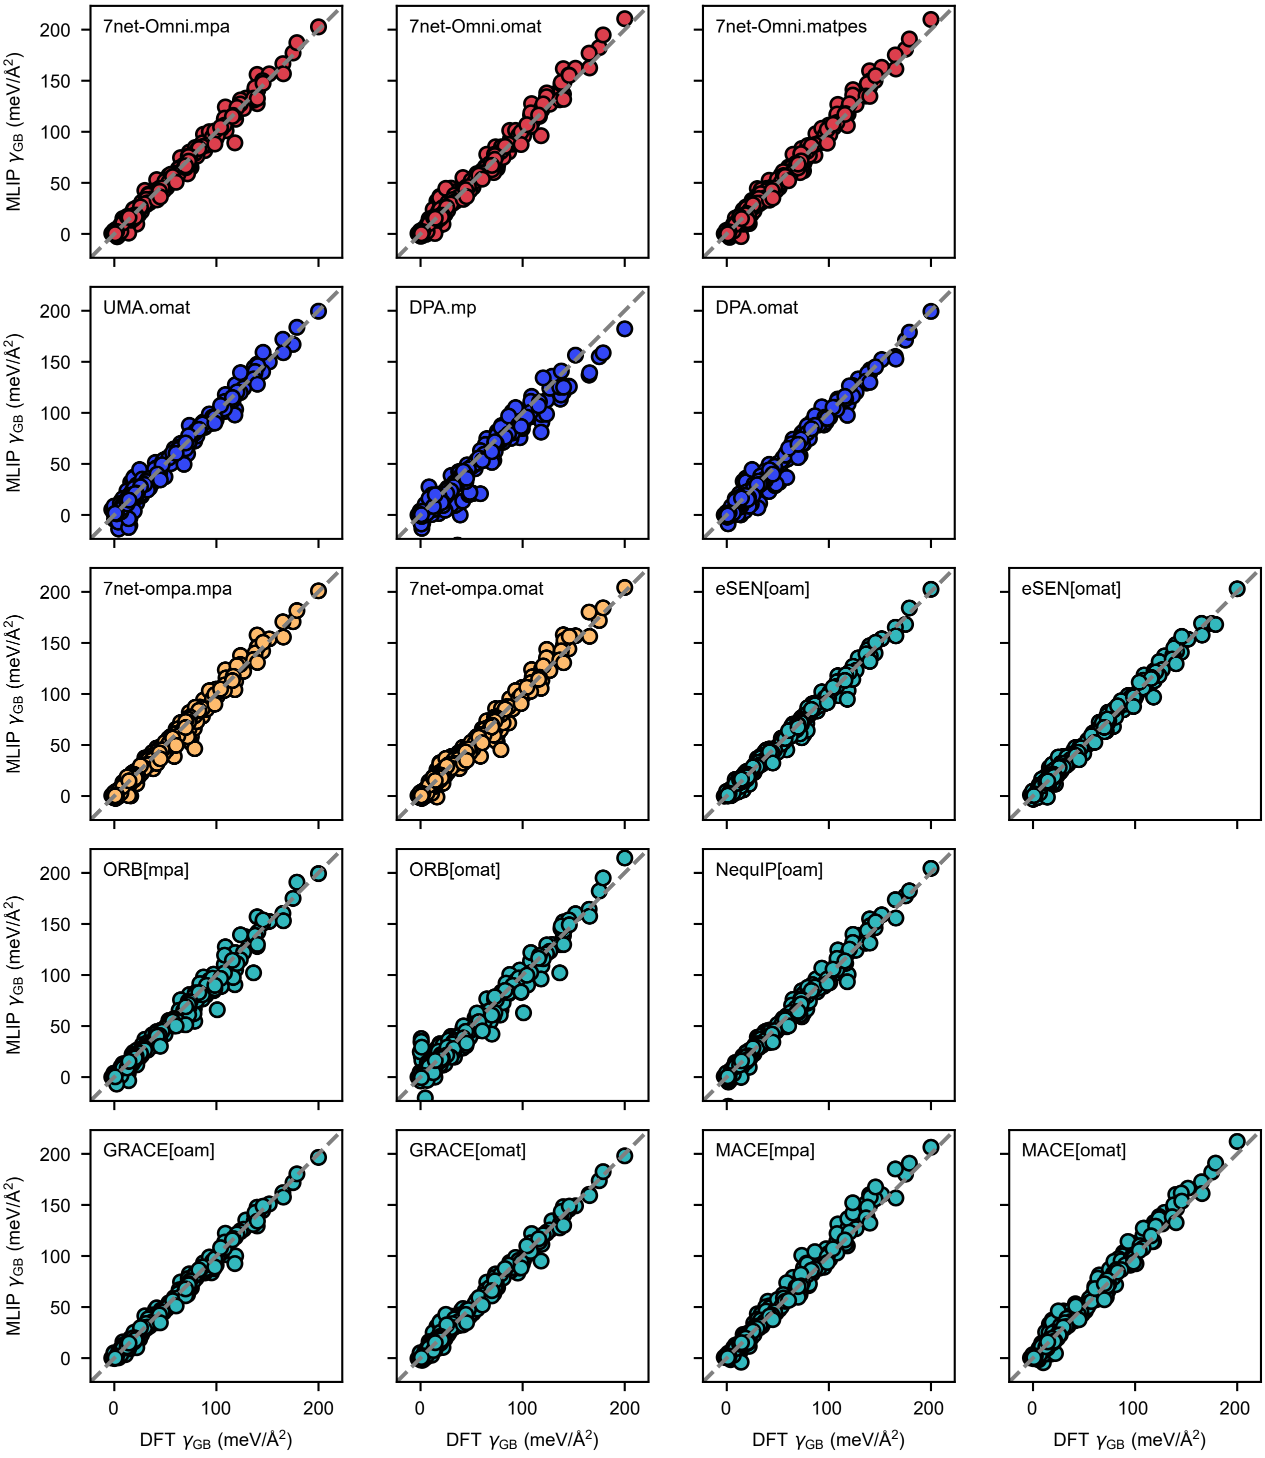


**Supplementary Figure 3: Party plots of grain boundary energies of elemental metals.** Reference values are calculated using PBE functional.

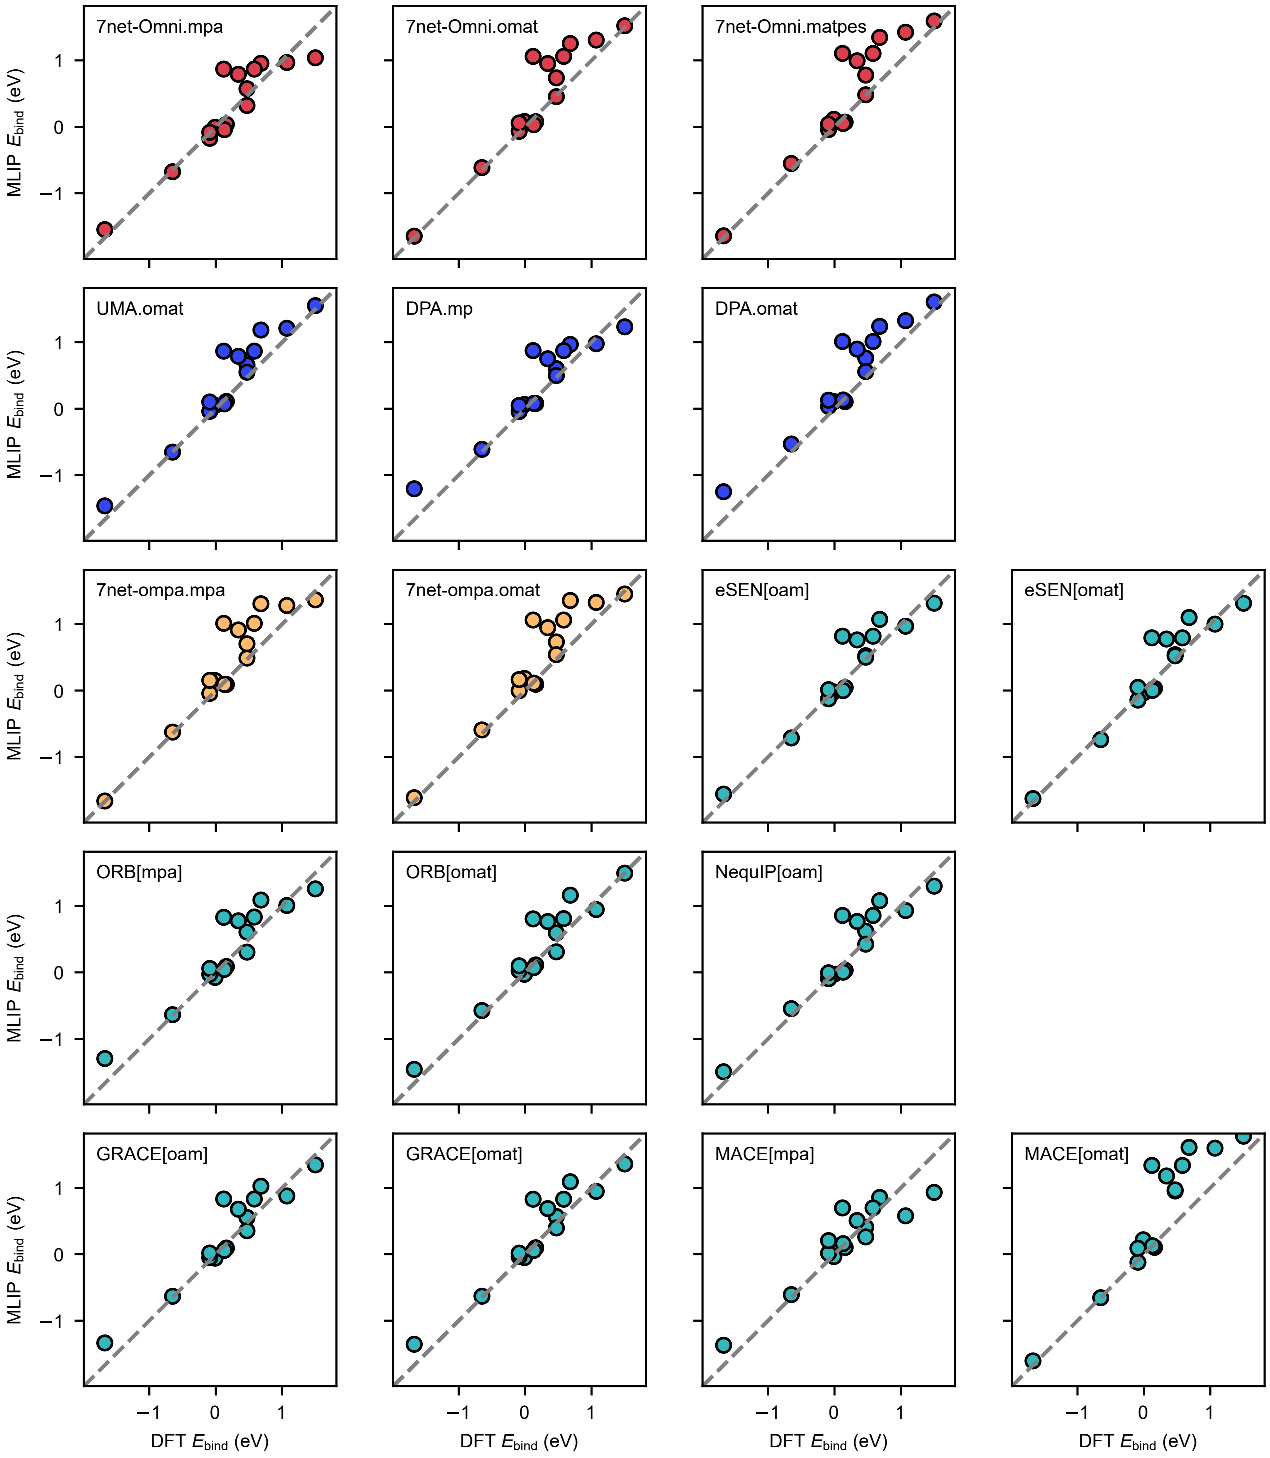


**Supplementary Figure 4: Party plots of binding energies between carbon interstitials and vacancies in steels.** Reference values are calculated using PBE functional.

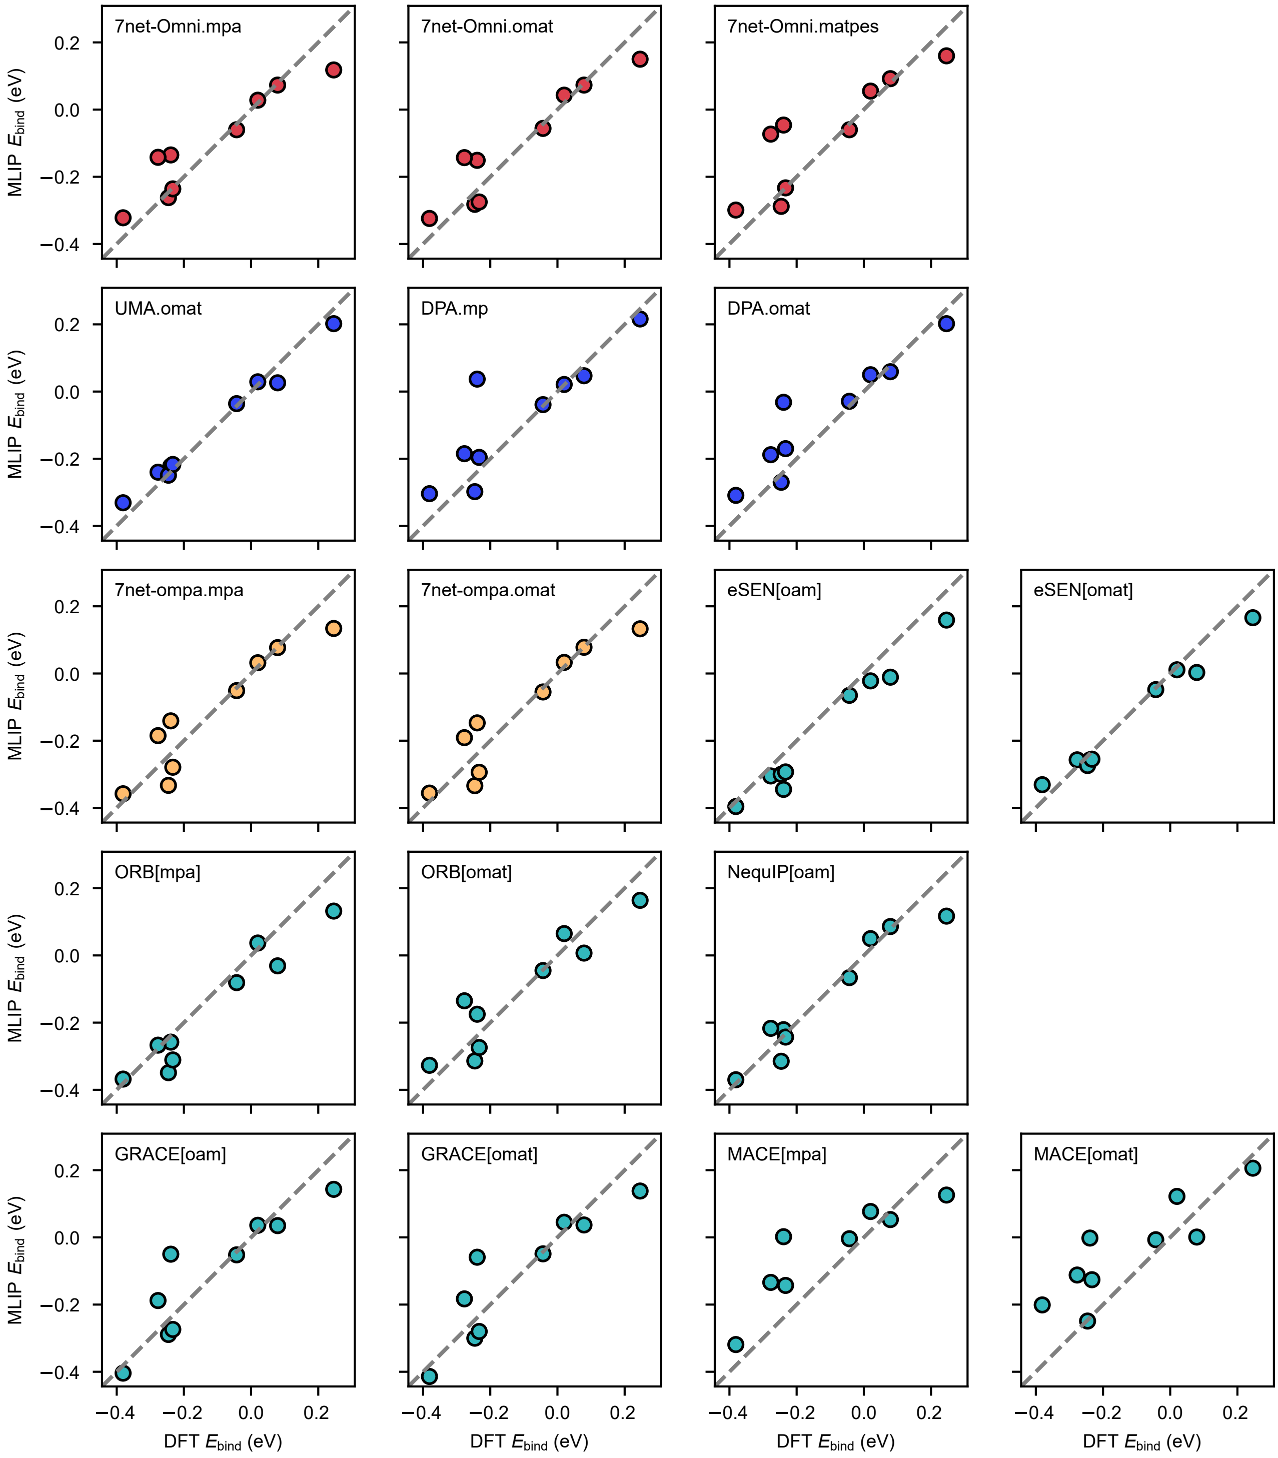


**Supplementary Figure 5**: **Party plots of binding energies between transition metal solutes in steels.** Reference values are calculated using PBE functional.

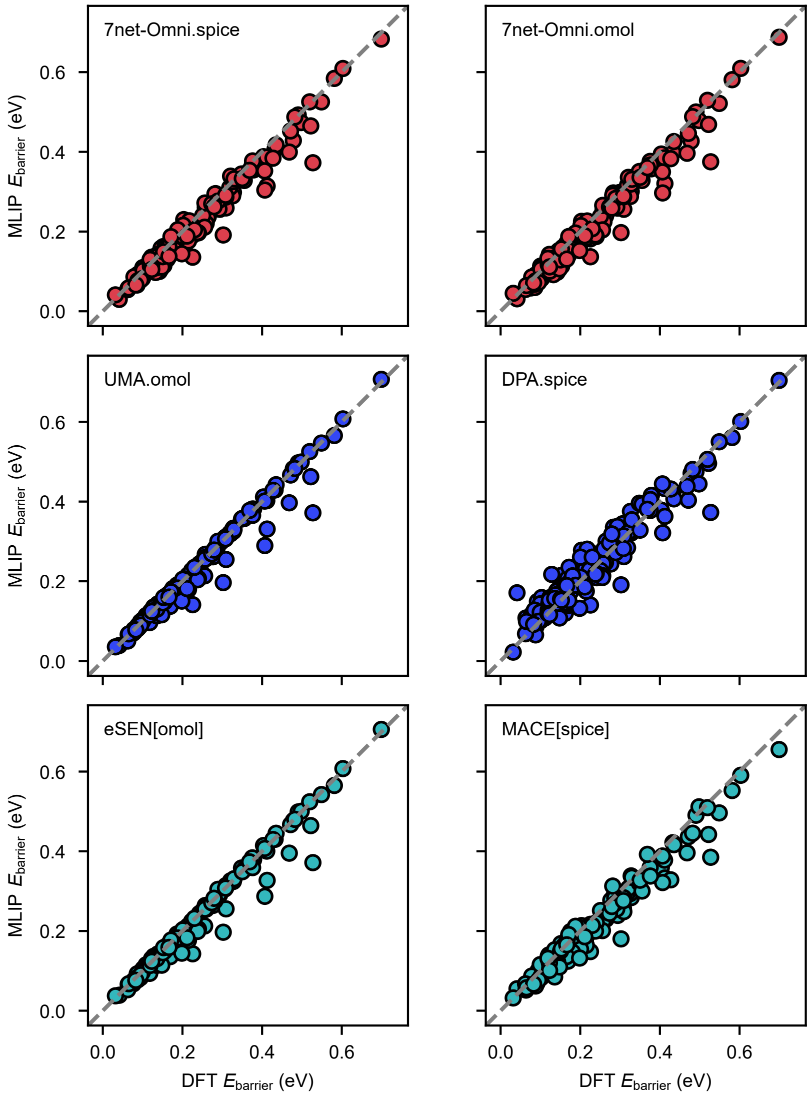


**Supplementary Figure 6**: **Party plots of torsion barrier energies in molecules.** Reference values are calculated using $\omega$B97M-D3 level of theory.

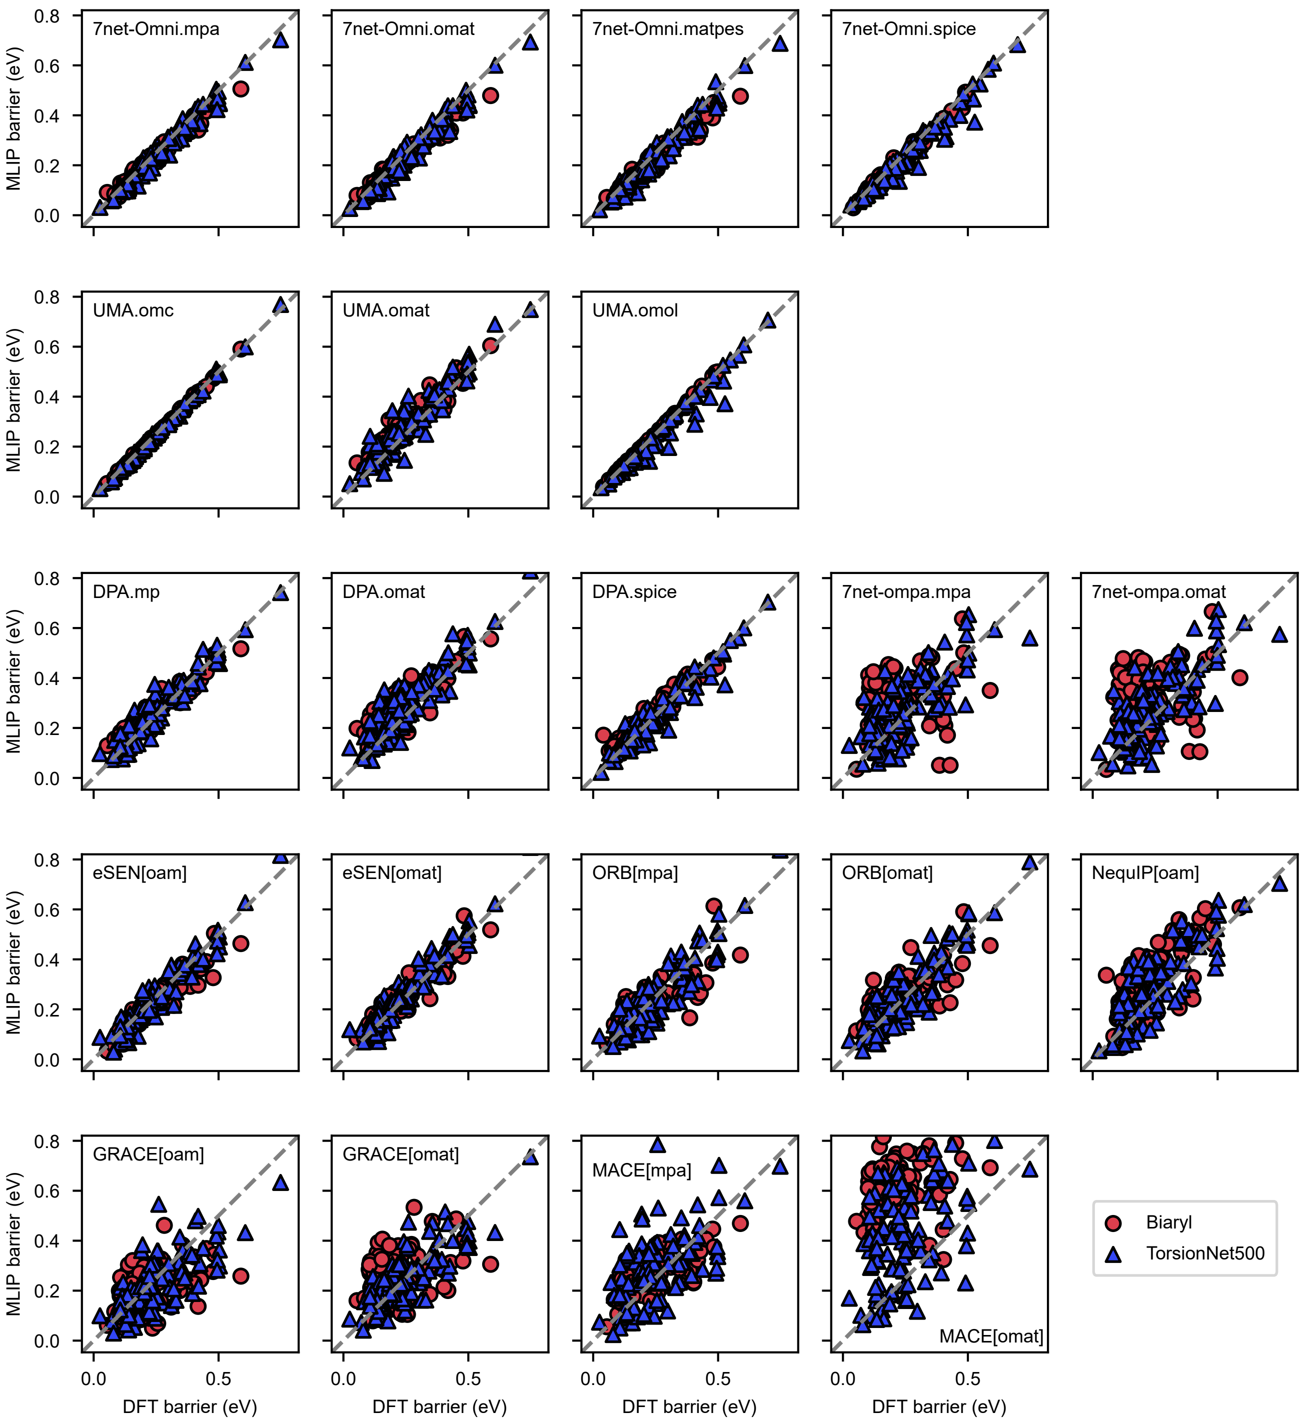


**Supplementary Figure 7**: **Party plots of torsion barrier energies in molecules.** Reference values are calculated at the PBE-D3 level of theory, except for MLIPs employing hybrid-fidelity channels (e.g., 7net-Omni.spice), for which the $\omega$B97M-D3 reference is used. Markers indicate the source of benchmark set at each data point (Biaryl or TorsionNet500).

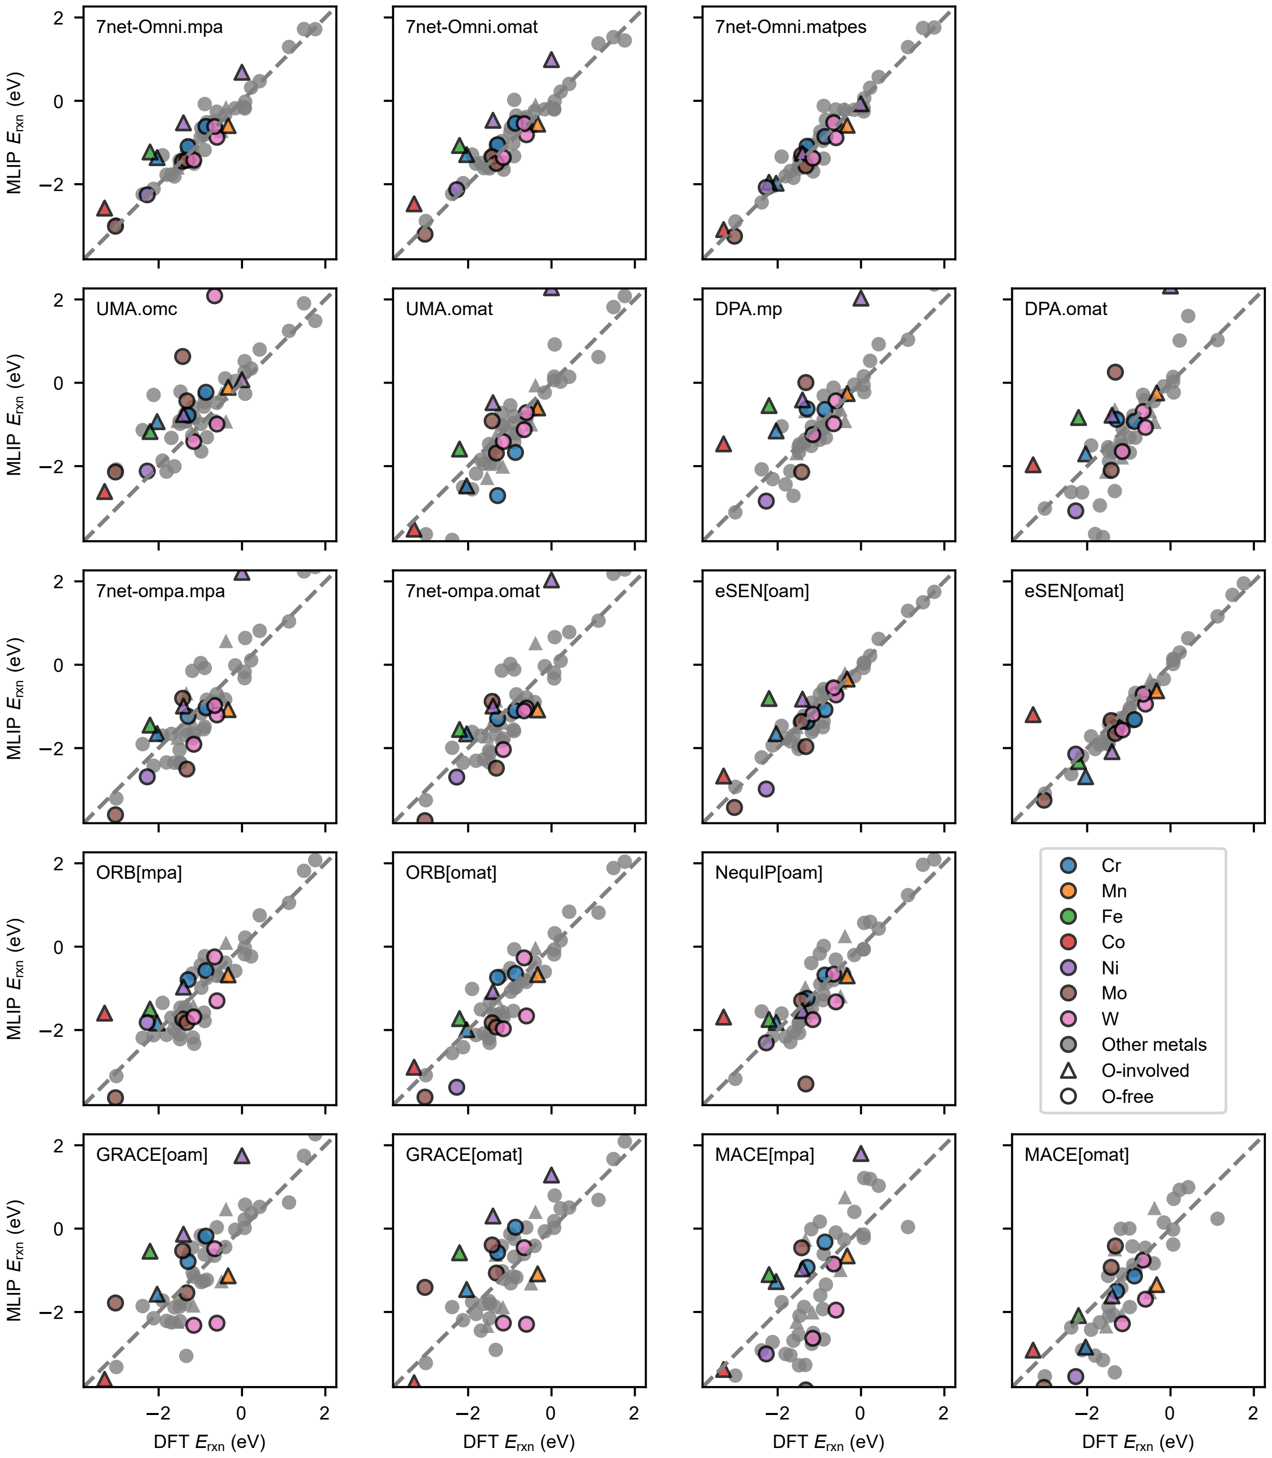


**Supplementary Figure 8**: **Party plots of reaction energies on organometallic reaction benchmark.** Reference values are calculated at the PBE-D3 level of theory. Non-gray colors indicate reactions involving center metals for which Hubbard $U$ correction is applied in the MPtrj/sAlex database, while other metals are shown in gray. Reactions where an oxygen atom is newly introduced near the center transition metal atom in the products are labeled as 'O-involved' (e.g. CO bonding to a core metal atom), whereas reactions in which the number of oxygen atoms near the metal center remains unchanged are labeled as 'O-free', The predictive accuracy exhibits metal-dependent variations, with O-involved reactions at Ni, Cr, Fe, and Co centers showing relatively large deviations in reaction energies in 7net-Omni.mpa. In constrast, matpes channel presents more uniform accuracy across the metal centers.

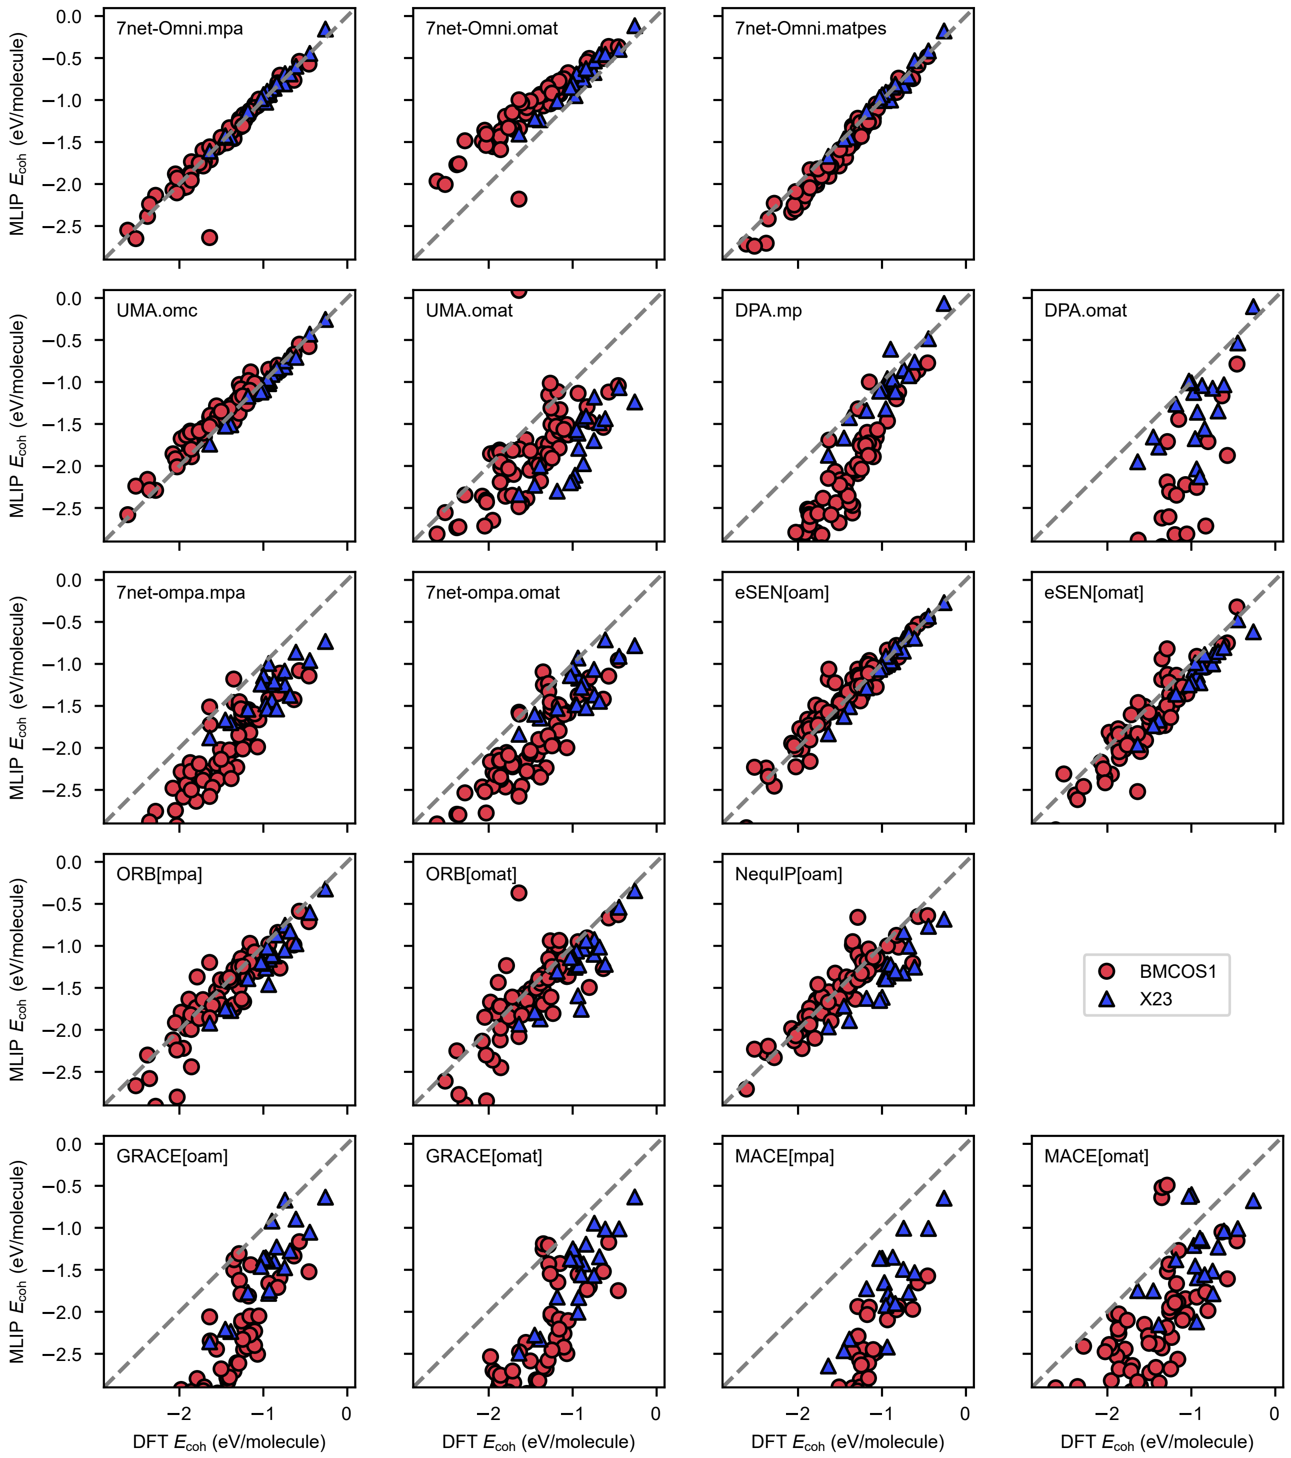


**Supplementary Figure 9**: **Party plots of cohesive energies of molecular crystals.** Reference values are calculated at the PBE-D3 level of theory. Markers indicate the source of benchmark set at each data point (BMCOS1 or X23).

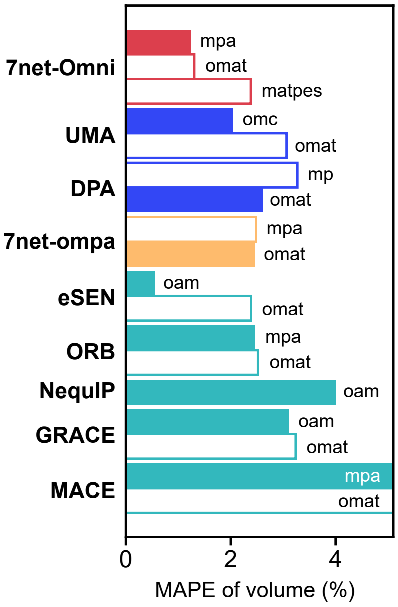


**Supplementary Figure 10**: **Volume prediction results for molecular crystals.** Mean absolute percentage errors (MAPEs) of volume predictions by uMLIPs for 86 molecular crystals in the X23 and BMCOS1 benchmark sets. Parity plots for each uMLIP are presented in Supplementary Fig. 11

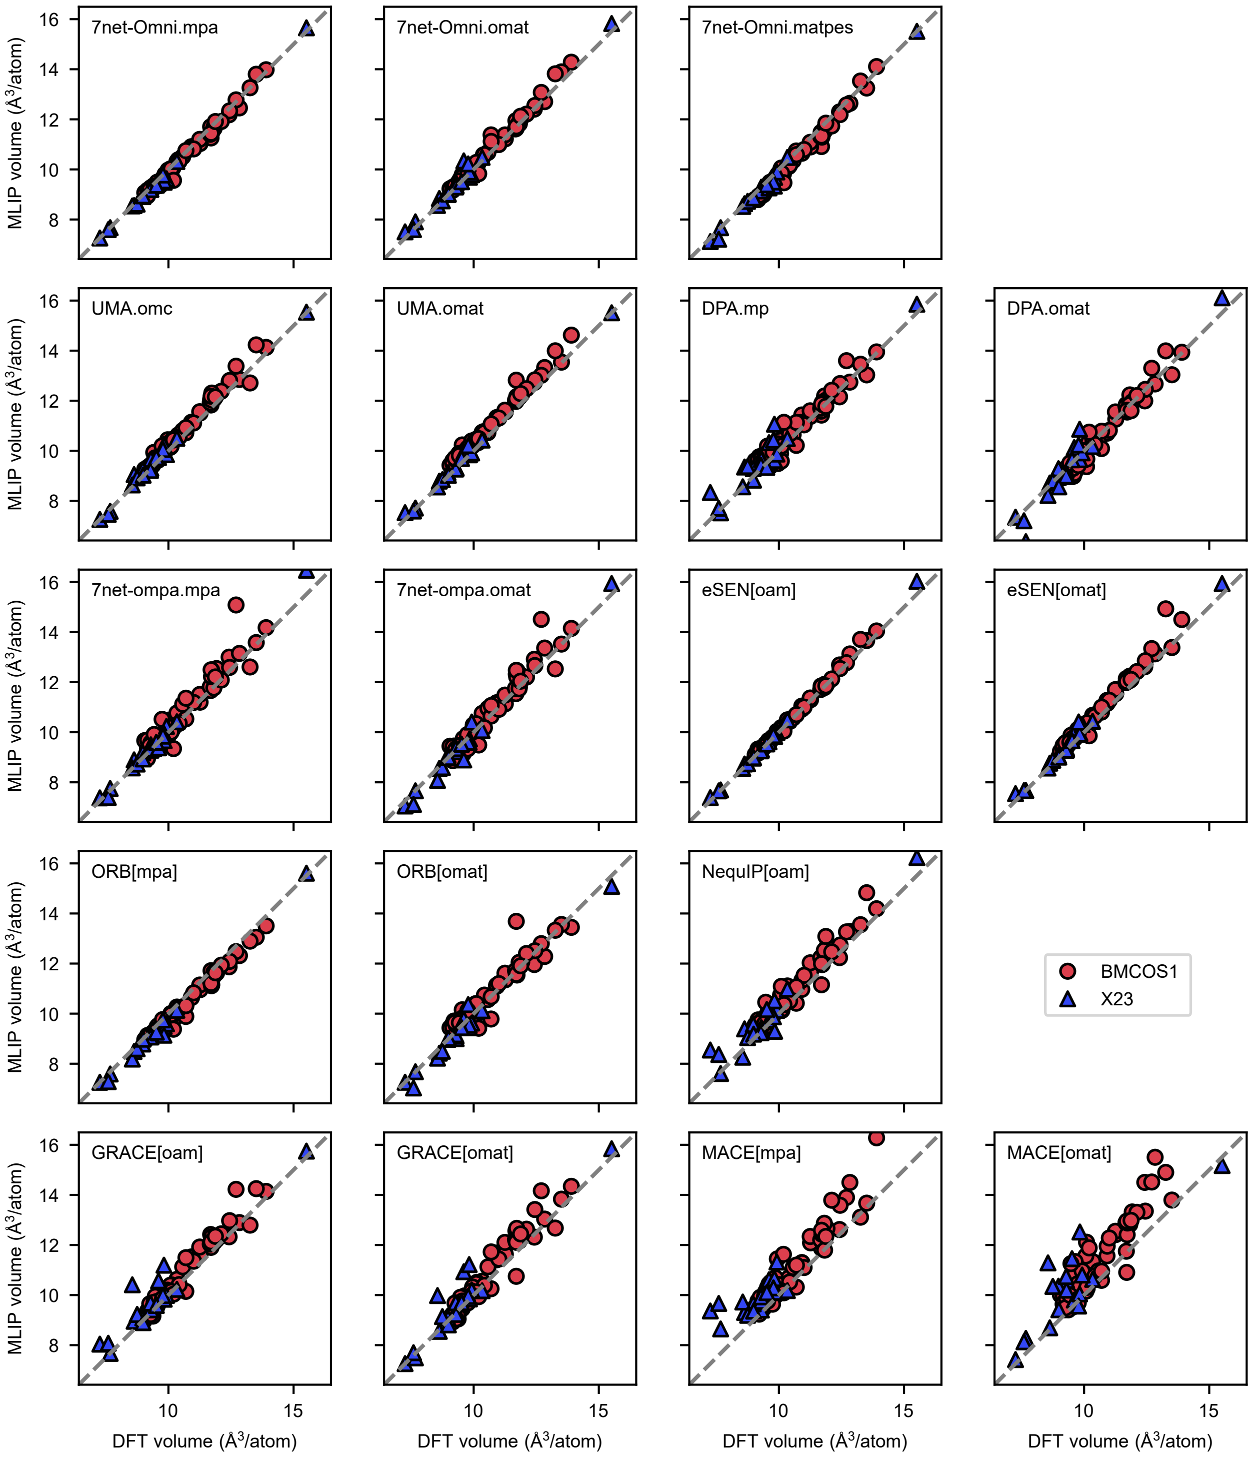


**Supplementary Figure 11**: **Party plots of equilibrium volumes of molecular crystals.** Reference values are calculated at the PBE-D3 level of theory. Markers indicate the source of benchmark set at each data point (BMCOS1 or X23).

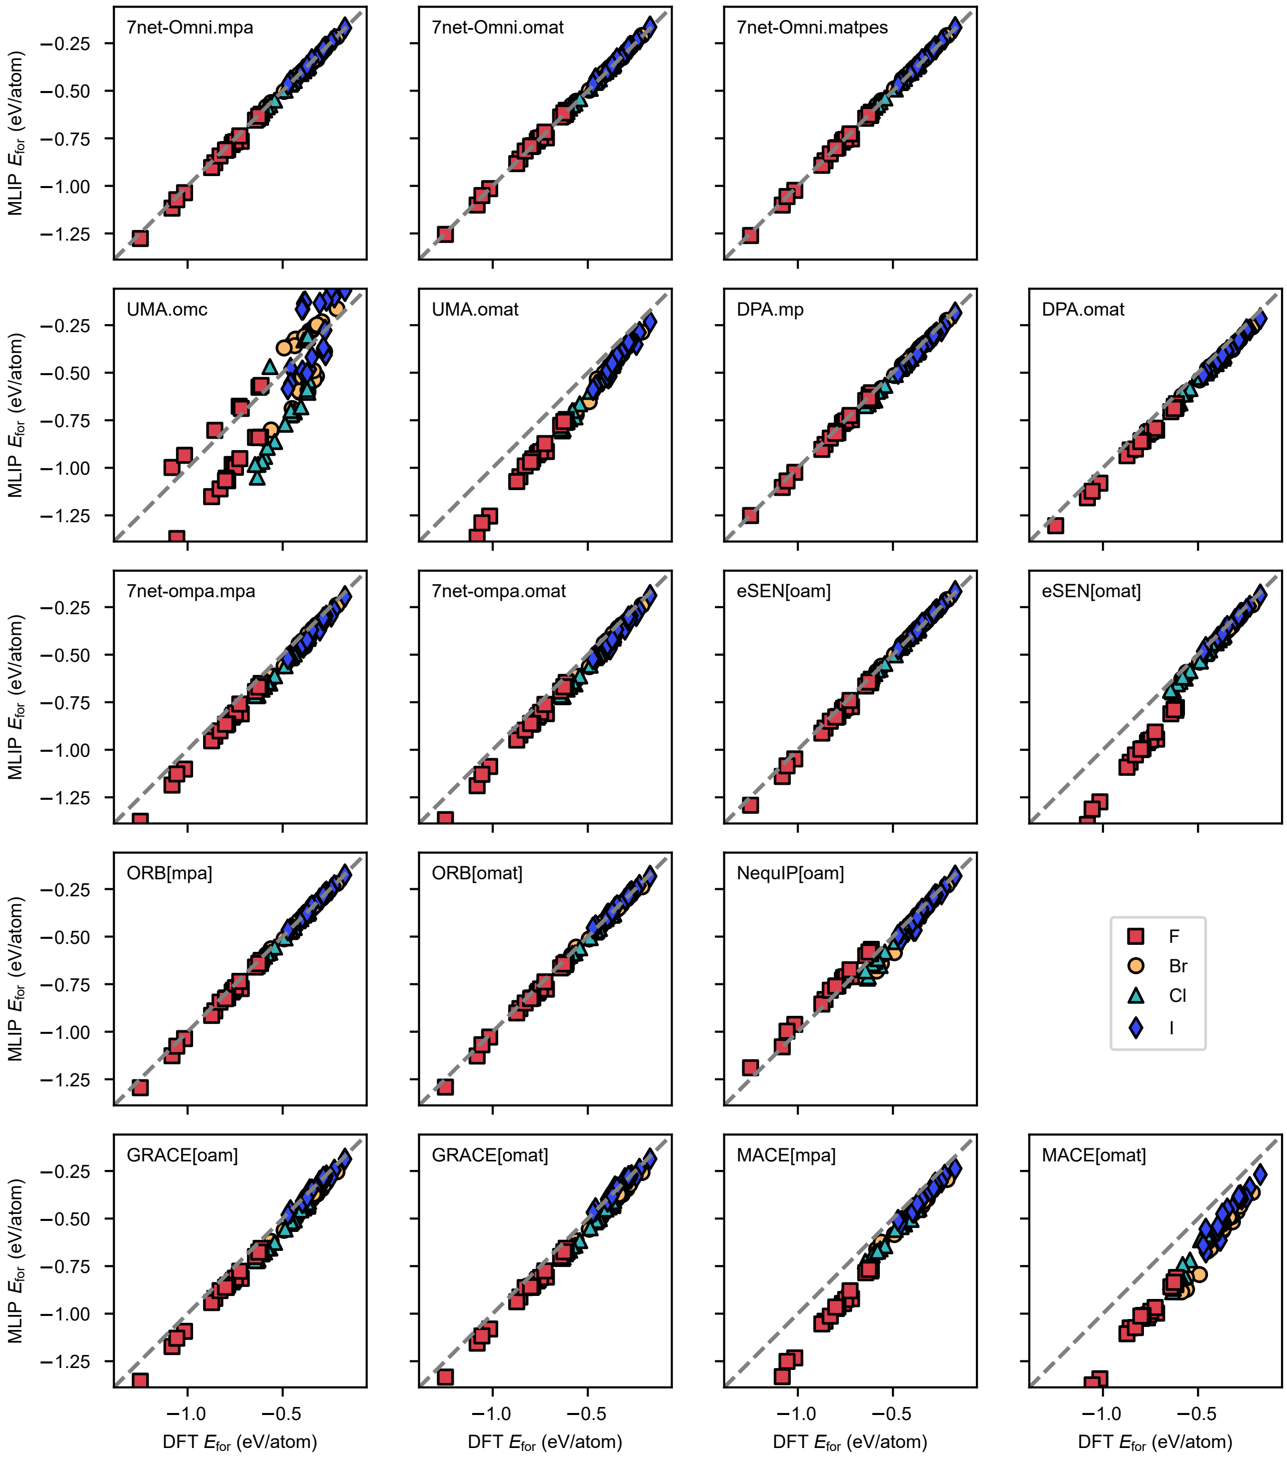


**Supplementary Figure 12**: **Party plots of relative energies of hybrid perovskites.** Reference values are calculated at the PBE-D3 level of theory. Markers indicate the halogen element contained in the perovskite.

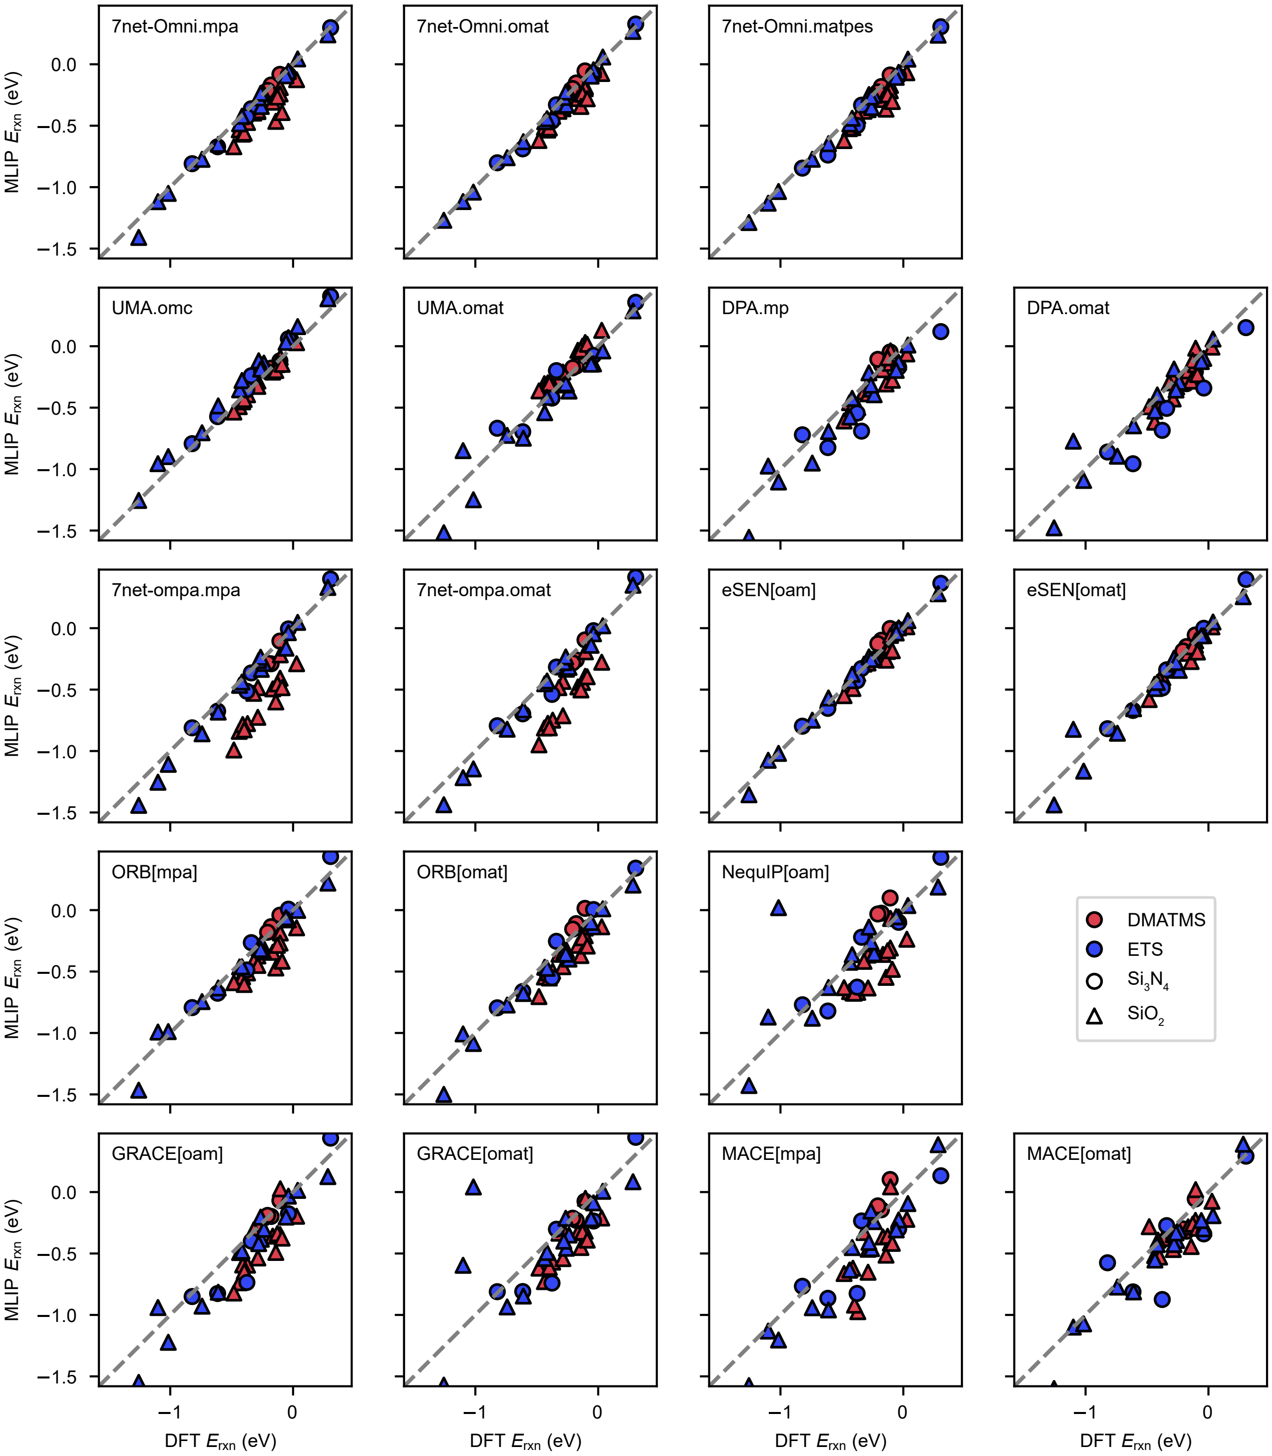


**Supplementary Figure 13**: **Party plots of reaction energies in area-selective deposition benchmark.** Reference values are calculated at the PBE-D3 level of theory. Color of each marker indicates the type of inhibitor molecule, while circle and triangle marker corresponds to $Si_3N_4$ and $SiO_2$ surface, respectively.

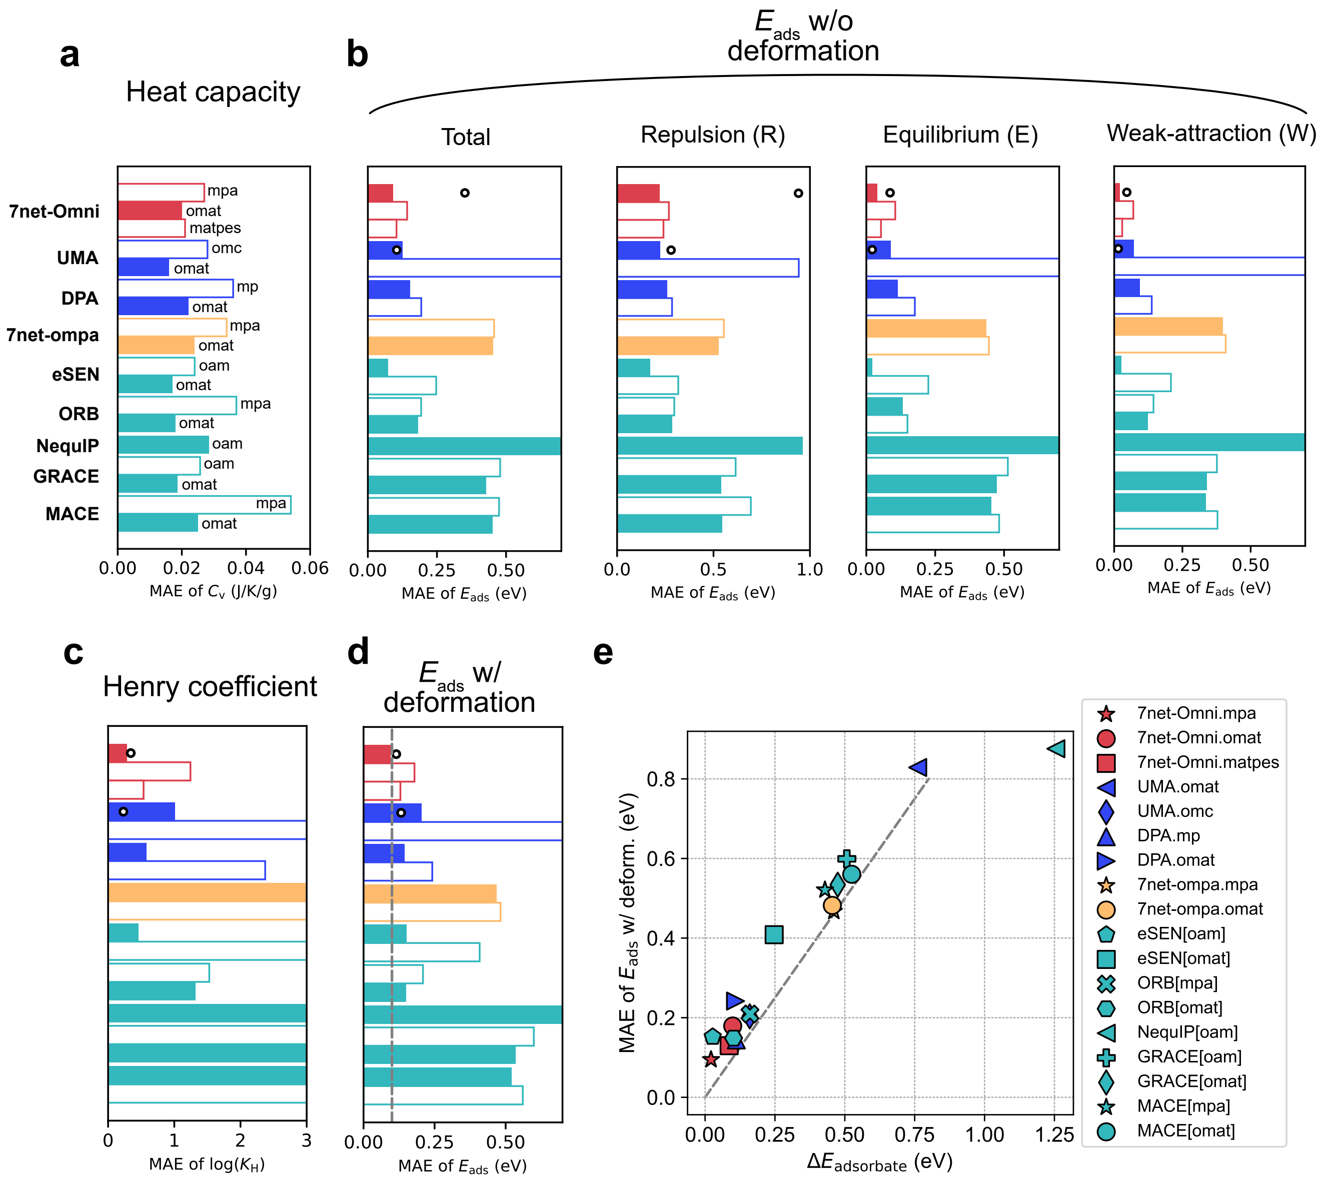


**Supplementary Figure 14: Benchmark tasks results for metal-organic frameworks. a** MAE of heat capacity. **b** MAE of adsorption energy without deformation. Since the GoldDAC dataset can be separated by its adsorption type, MAEs according to three different (repulsion, equilibrium, and weak-attractive) cases were displayed. **c** MAE of $CO_2$ henry coefficient. Logarithm value of henry coefficient were used for convenience. **d** MAE of adsorption energy with deformation. Gray dashed line denotes 0.1 eV. **e** The relationship between error in energy of adsorbate and MAE of adsorption energy with deformation. Gray dashed line denotes $y = x$. Bulltin points in Fig. **b-d** respectively denote 7net-Omni.odac23 and UMA.odac. Individual parity plots are presented in Supplementary Fig. 15 to 19.

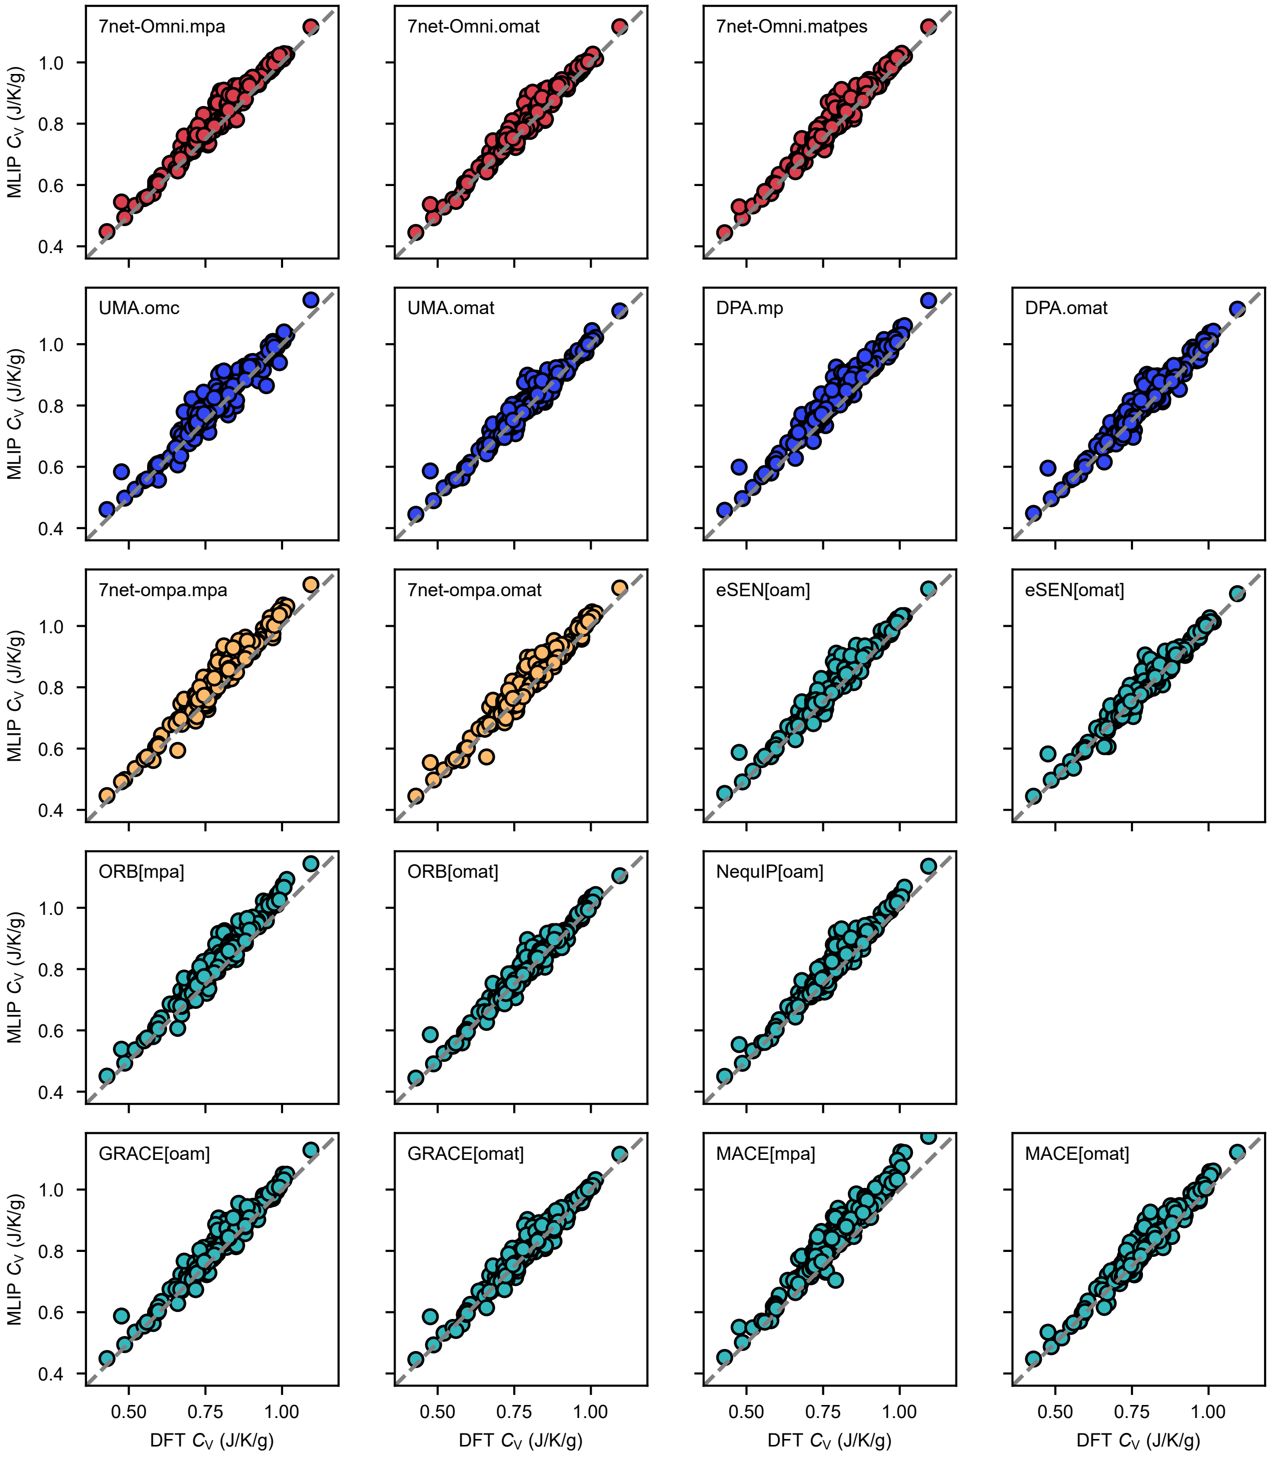


**Supplementary Figure 15**: **Party plots of heat capacities of MOFs.** Reference values are calculated at the PBE-D3 level of theory.

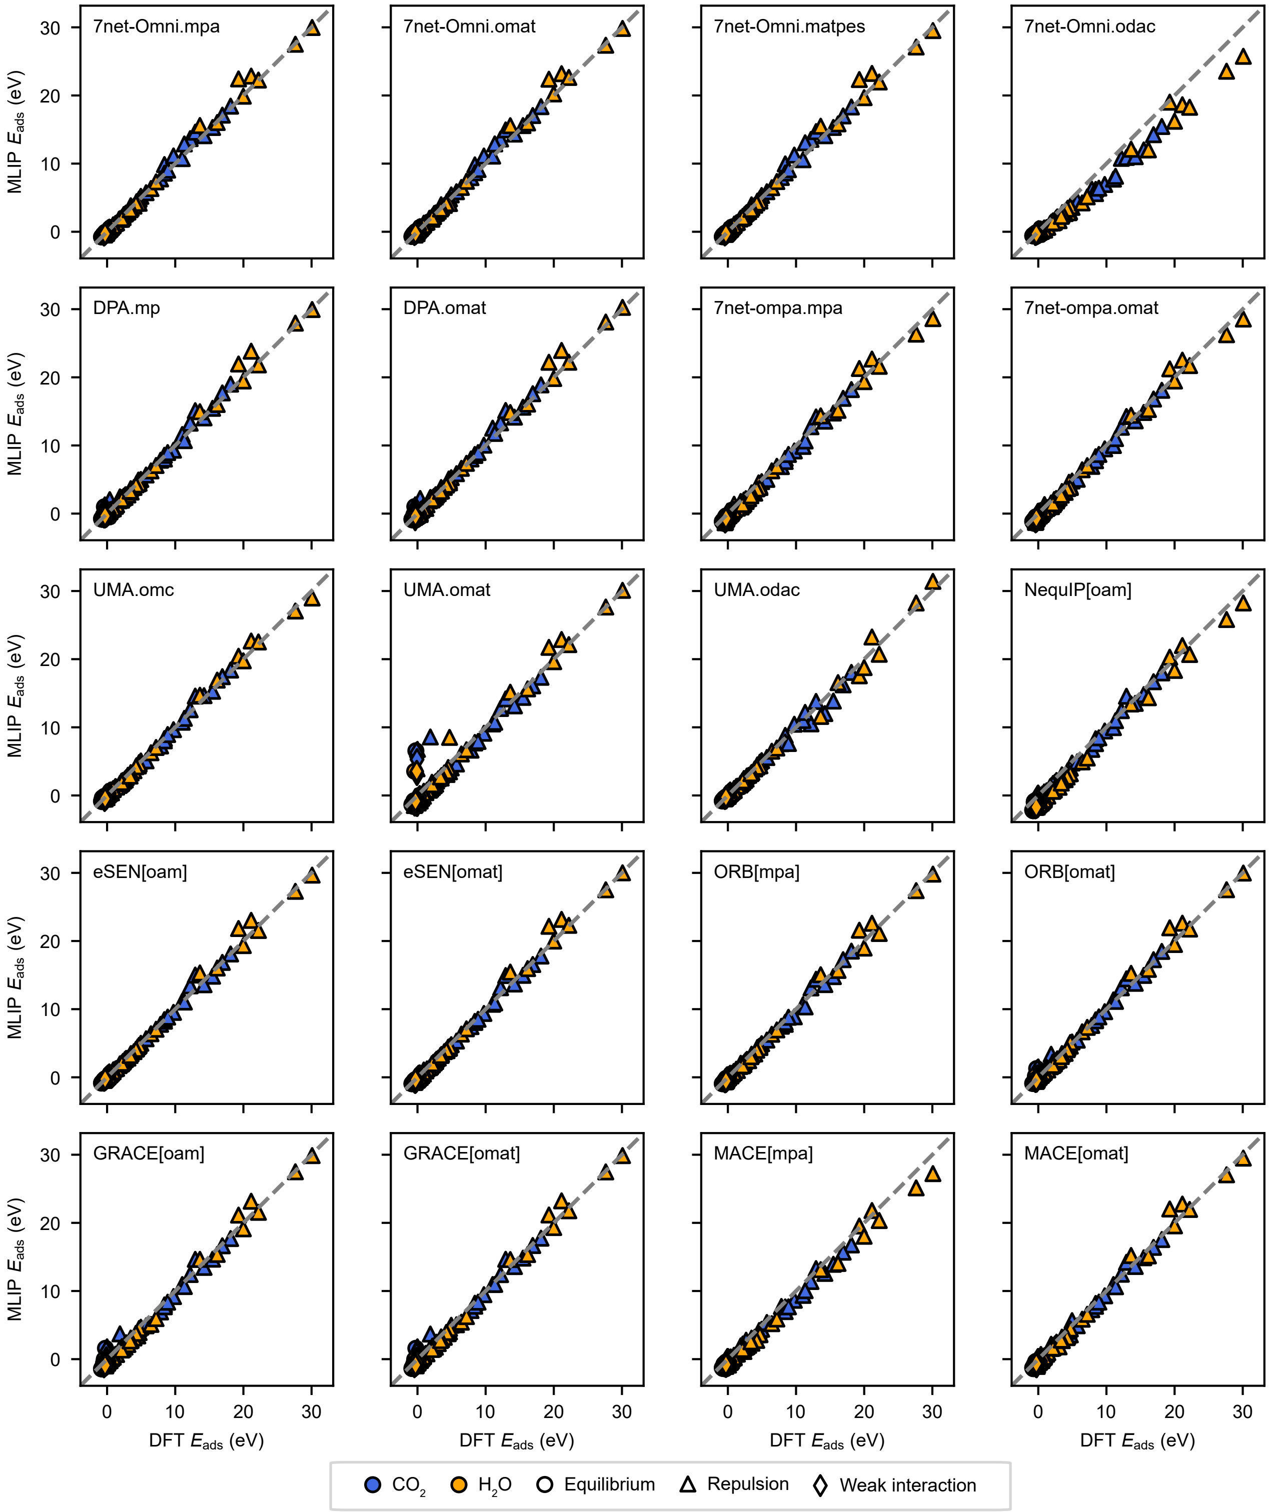


**Supplementary Figure 16**: **Party plots of adsorption energy of molecules in MOFs without relaxation.** Reference values are calculated at the PBE-D3 level of theory. Color of each marker indicates the type of molecule ($CO_2$ and $H_2O$), while circle, triangle and diamond marker corresponds to energy region of equilibrium, repulsion, and weak interaction, respectively.

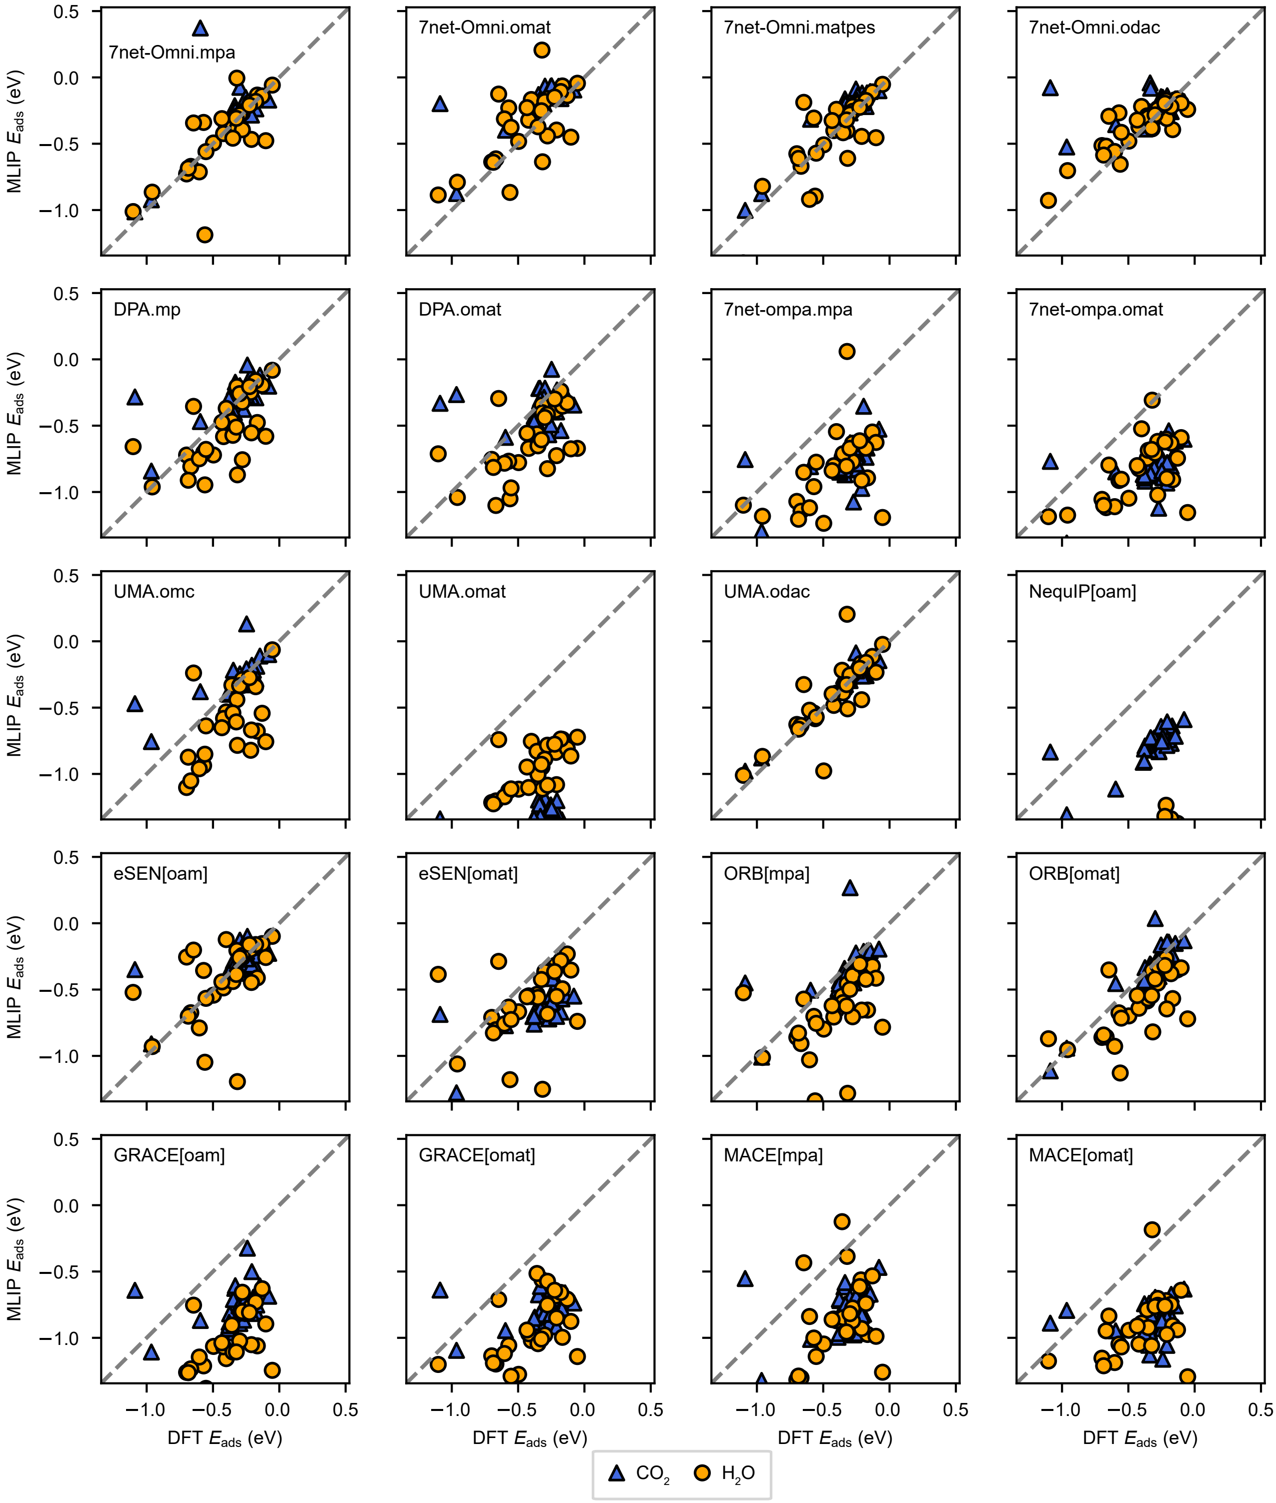


**Supplementary Figure 17**: **Party plots of adsorption energy of molecules in MOFs with relaxation.** Reference values are calculated at the PBE-D3 level of theory. Color of each marker indicates the type of molecule ($CO_2$ and $H_2O$) adsorbed to the MOF.

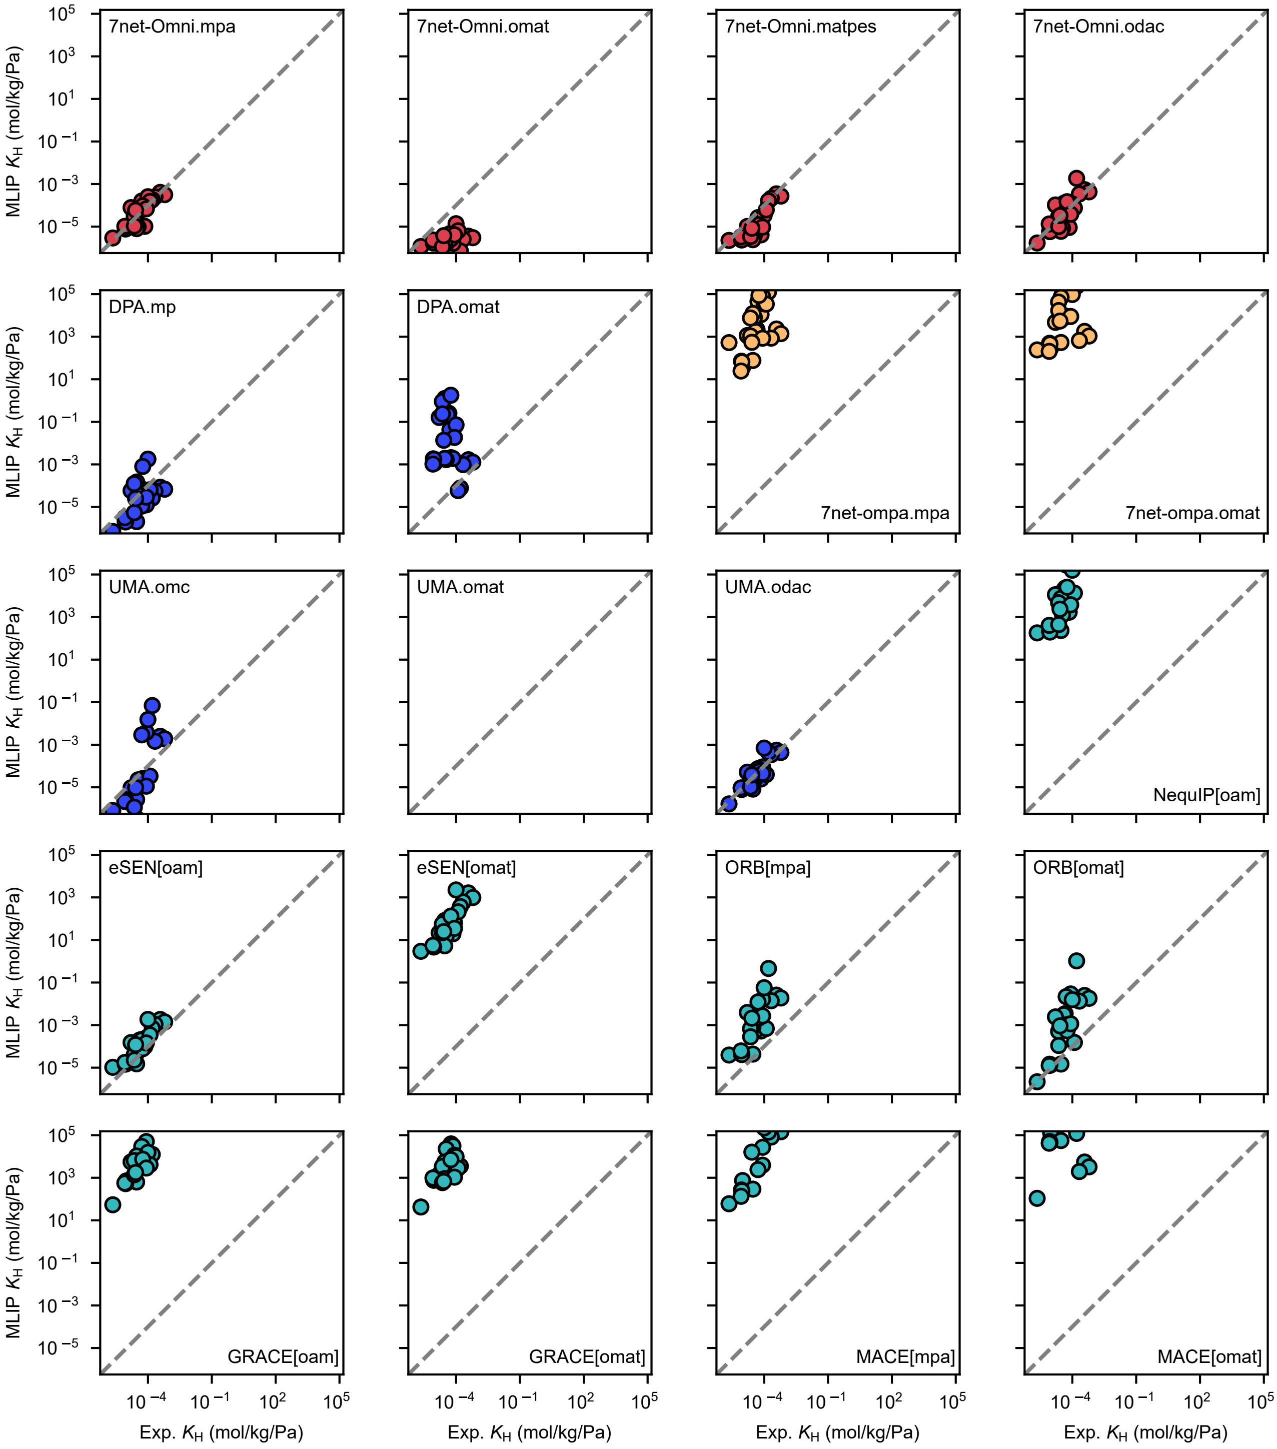


**Supplementary Figure 18**: **Party plots of Henry coefficients of MOFs.** Reference values are obtained by experiment.

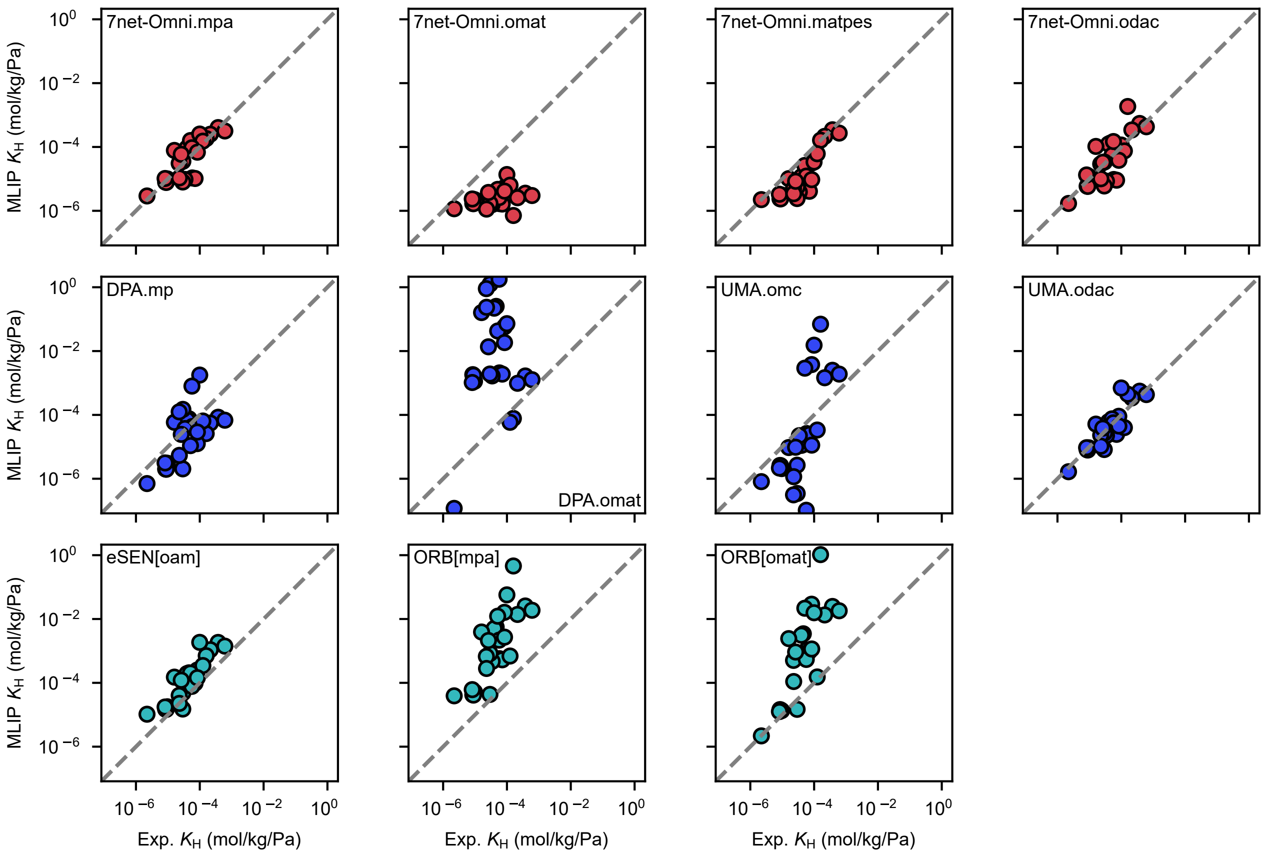


**Supplementary Figure 19: Party plots of Henry coefficients of MOFs, only showing MLIPs that give reasonable range of results.** Reference values are obtained by experiment.

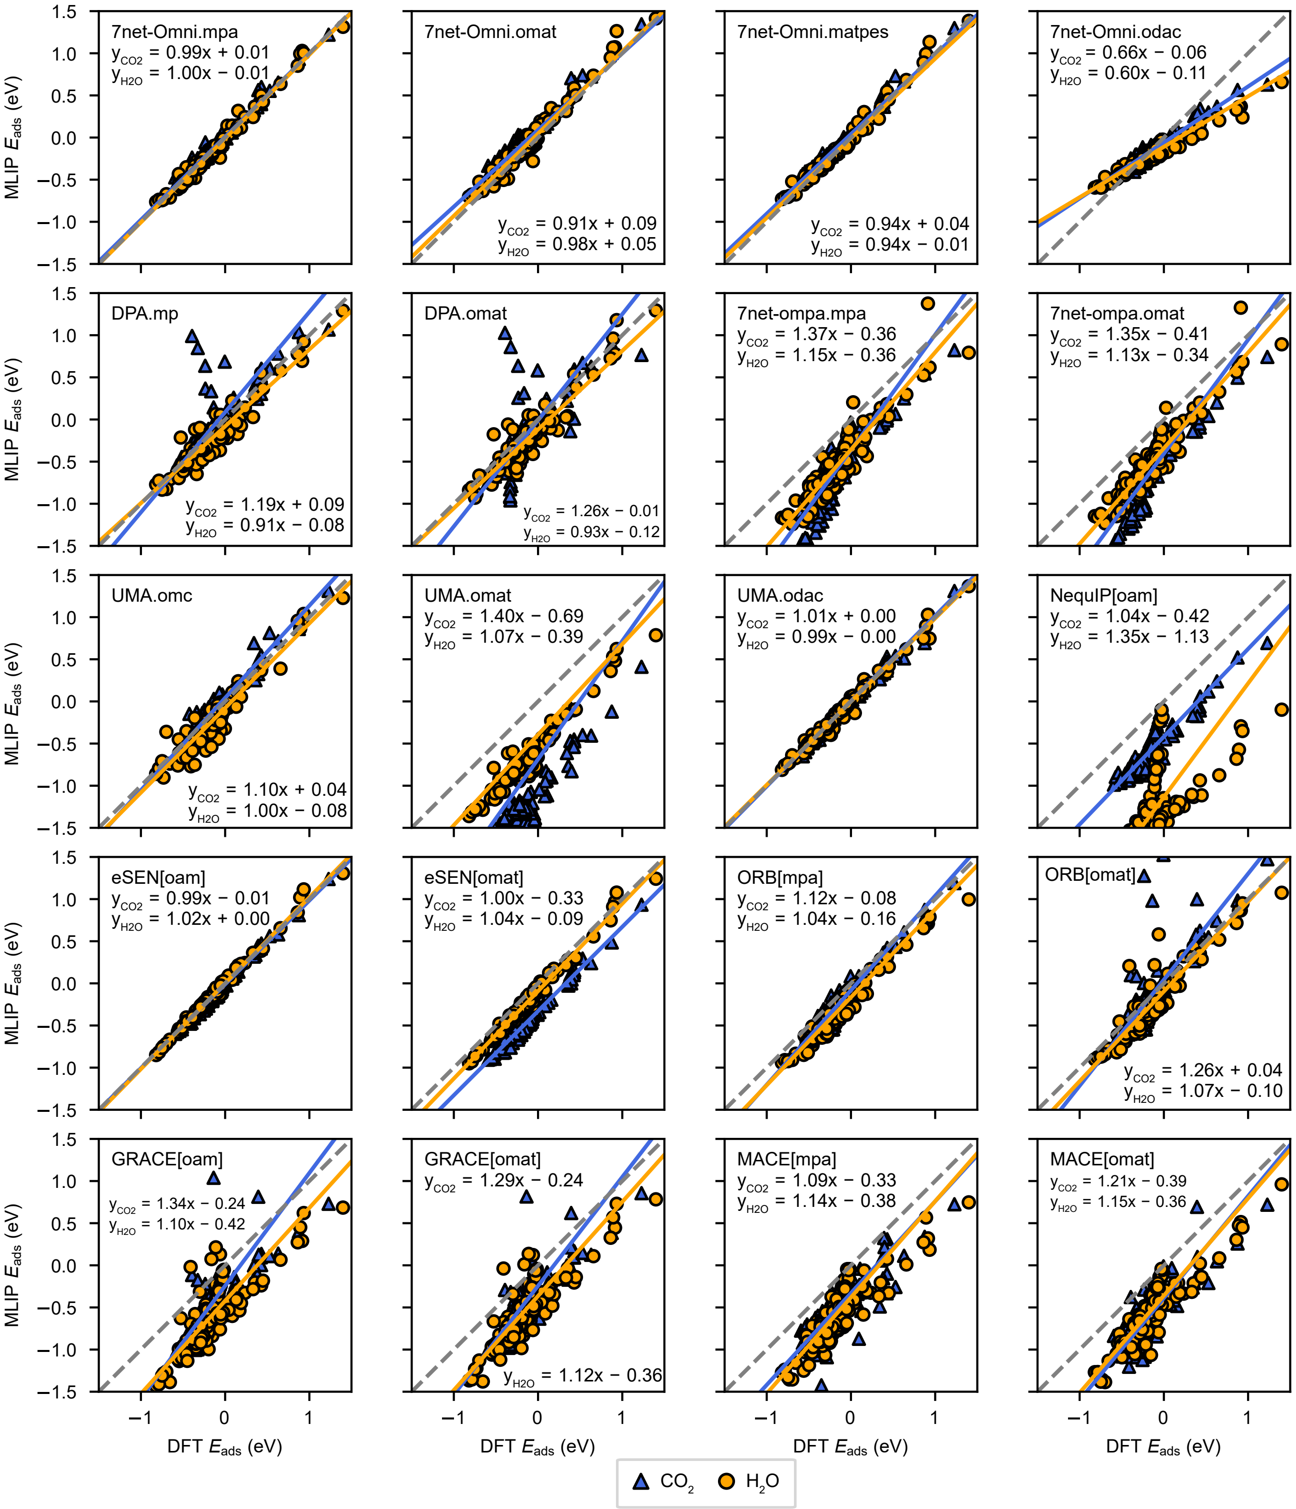


**Supplementary Figure 20**: **Party plots of adsorption energy of molecules in MOFs without relaxation, enlarged to the energy region under 1.5 eV.** Reference values are calculated at the PBE-D3 level of theory. Blue and orange lines indicate linear regression line fitted to the data points of DFT adsorption energy less than 0.5 eV, corresponds to $CO_2$ and $H_2O$, respectively.

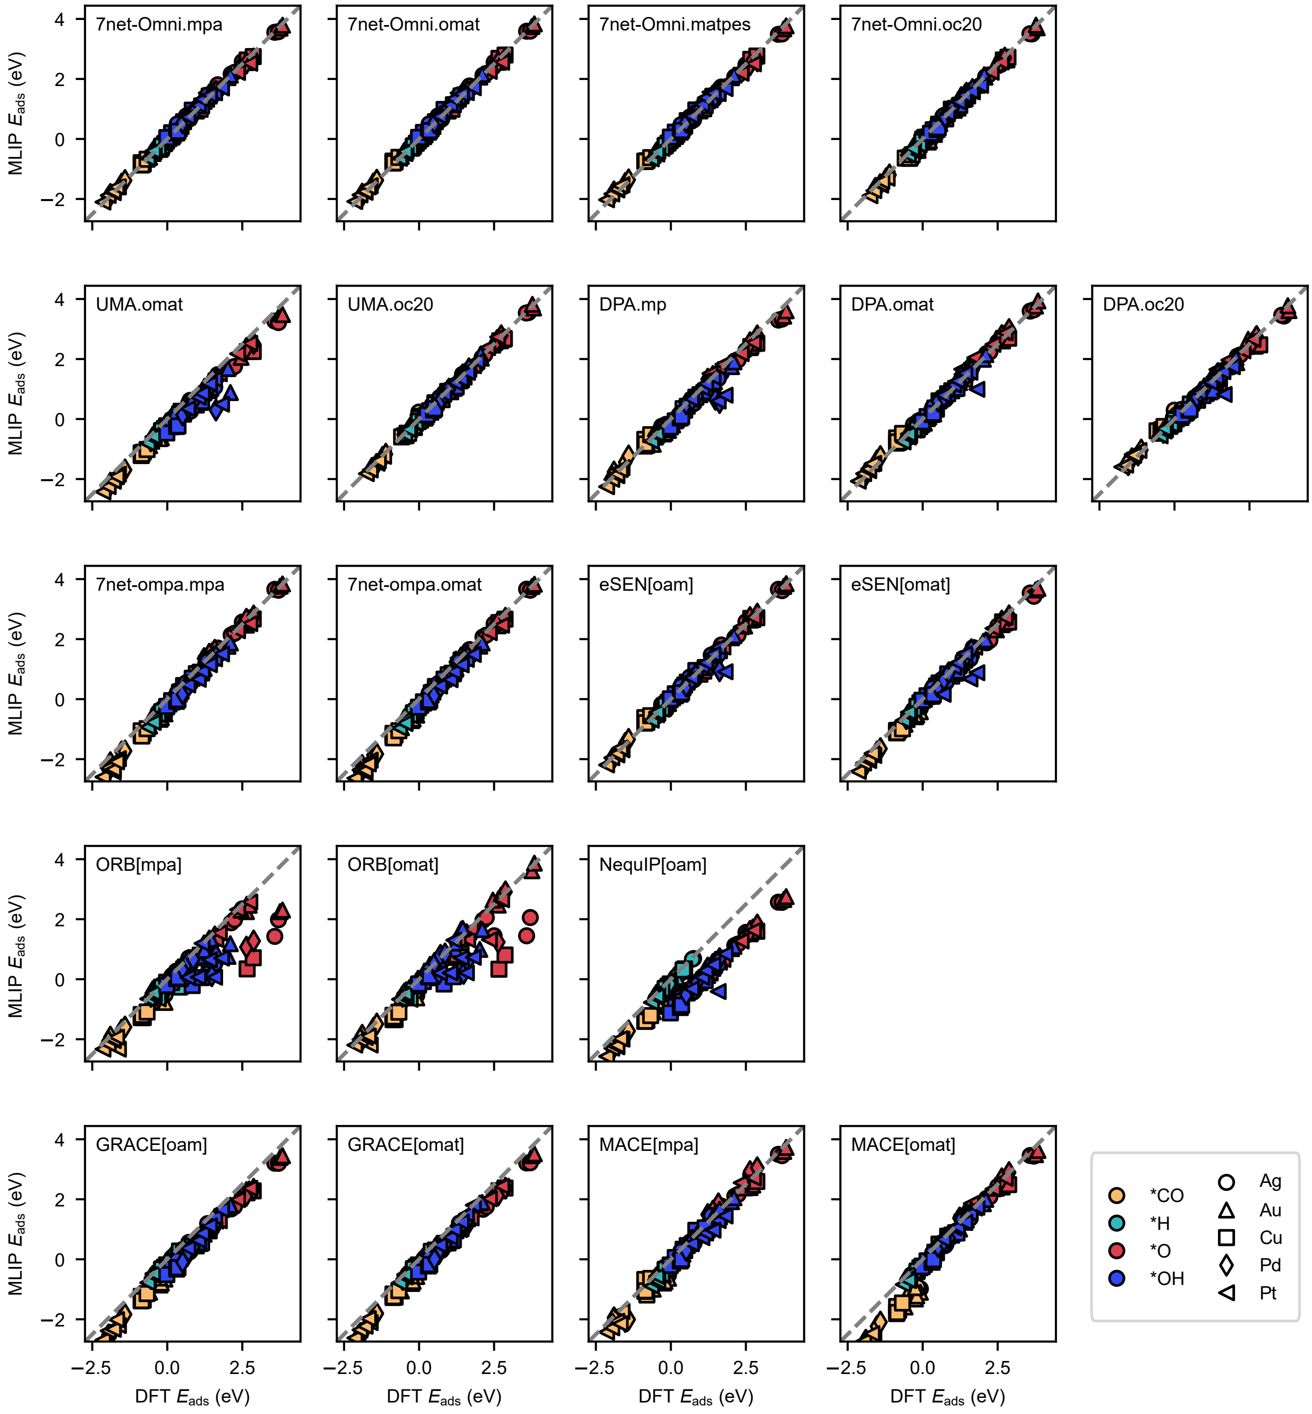


**Supplementary Figure 21**: **Party plots of adsorption energies in noble metal surfaces.** Reference values are calculated with PBE functional except for MLIPs employing RPBE-fidelity channels (e.g., 7net-Omni.oc20), for which the RPBE reference is used. Color of each marker indicates the type of adsorbates, while shape of marker corresponds to the type of noble metal.

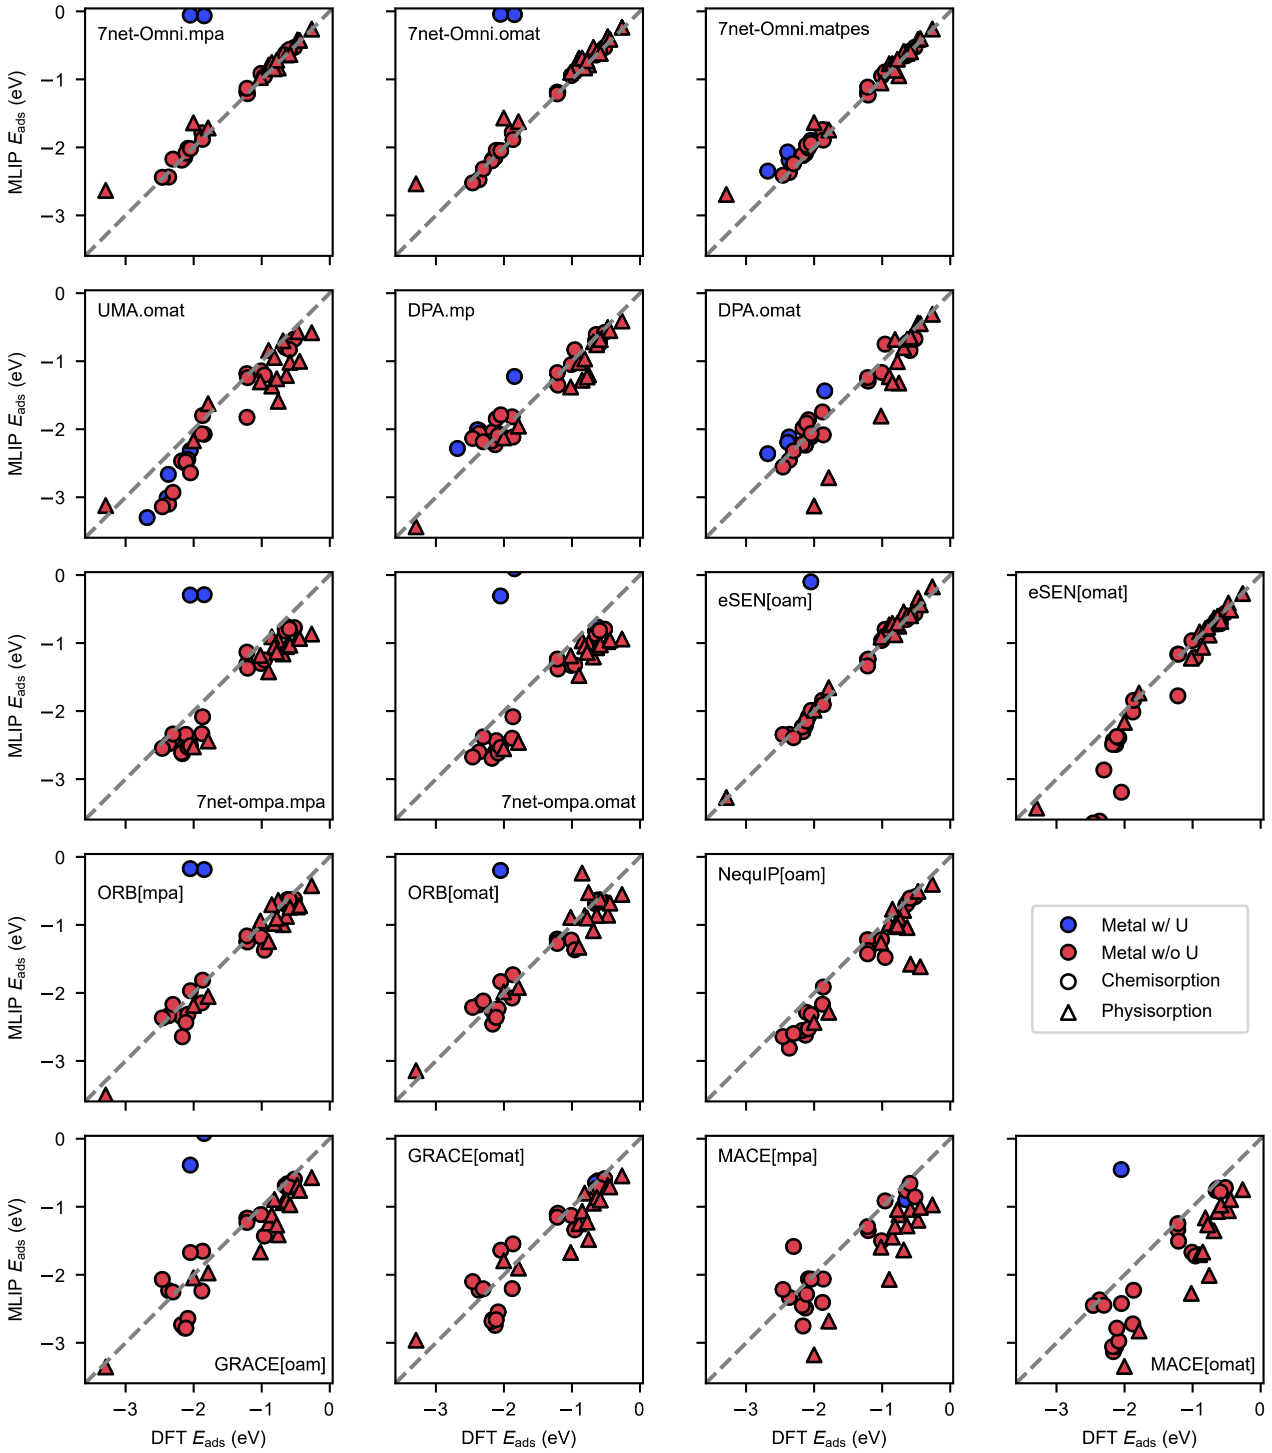


**Supplementary Figure 22**: **Party plots of adsorption energies in ADS41 benchmark.** Reference values are calculated with PBE-D3 level of theory. Color of marker indicates whether corresponding metal element utilizes Hubbard $U$ correction in MPtrj/sAlex database, while circle and triangle marker corresponds to chemisorption and physisorption, respectively.

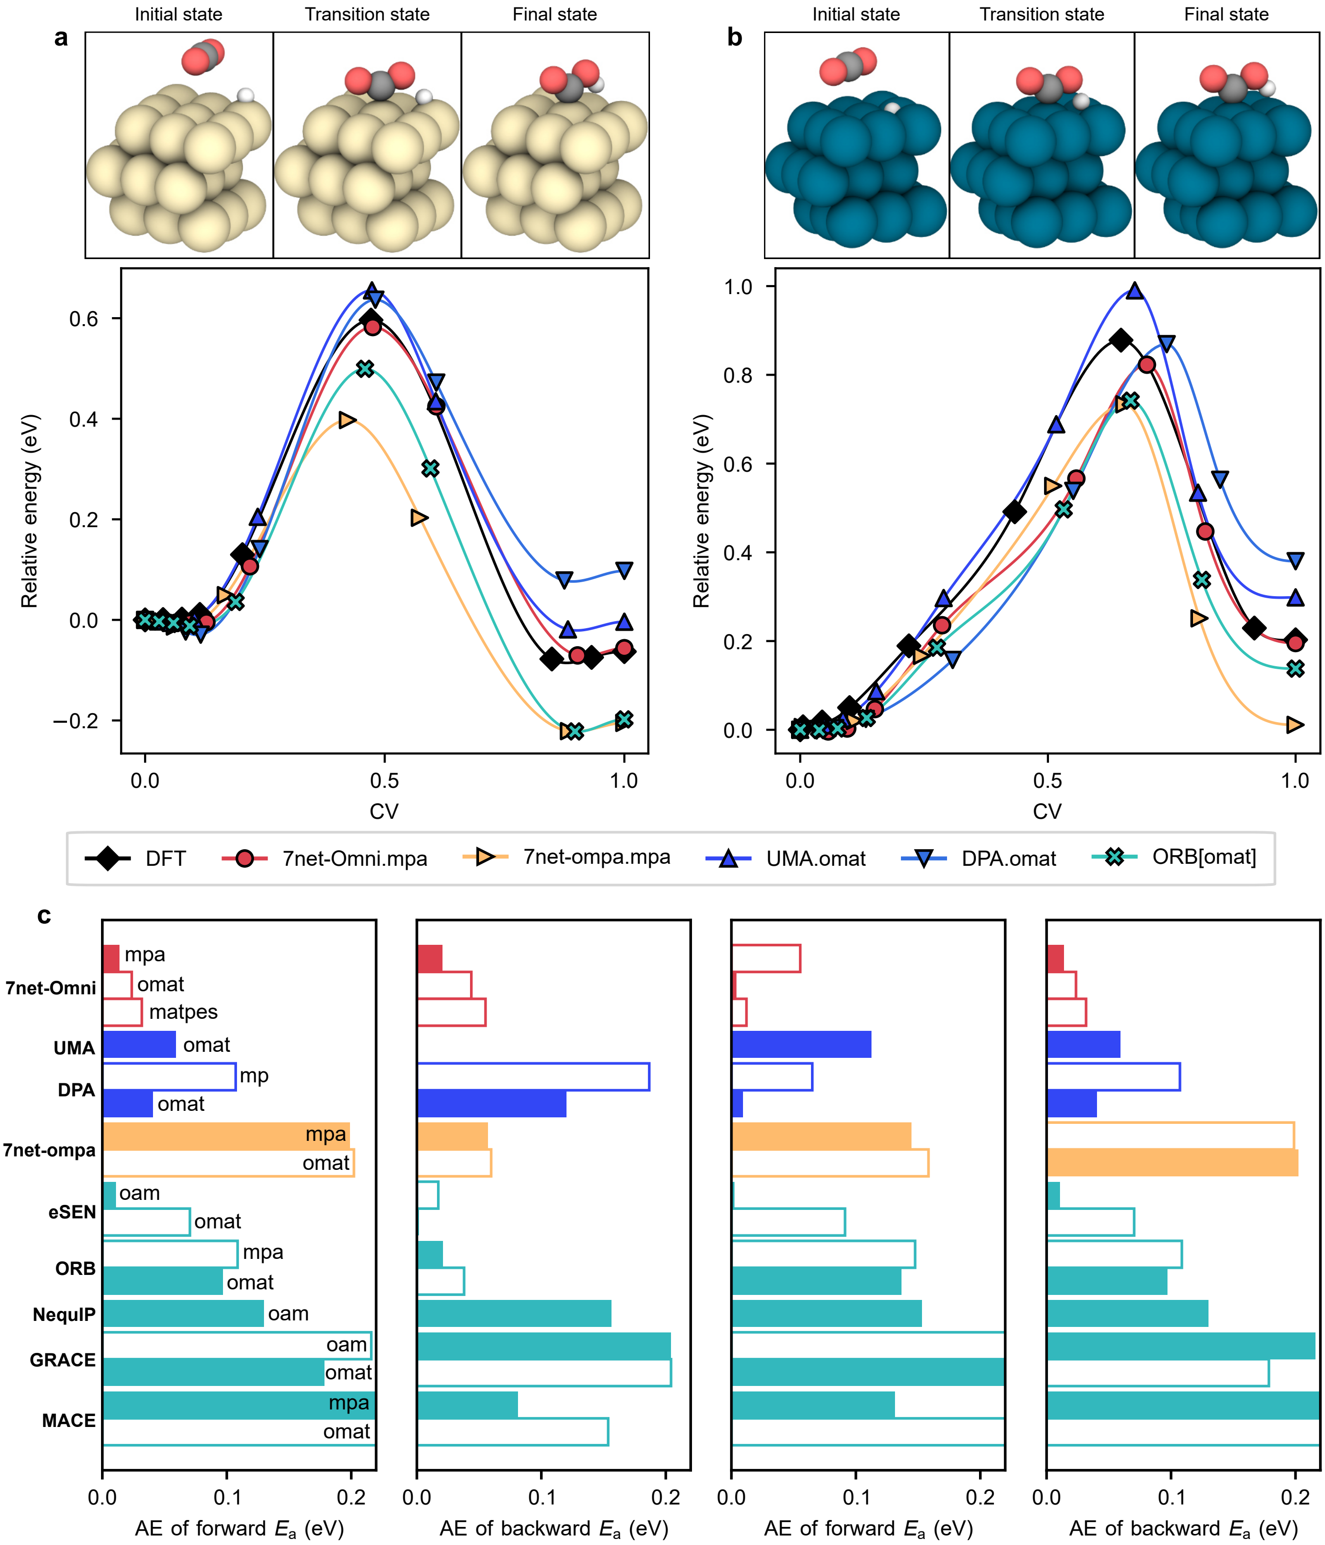


**Supplementary Figure 23**: **Benchmark results in $CO_2$RR on Pt and Pd surfaces. a** NEB calculation results in Pt (111) surface. PES are illustrated using collective variable (CV) based on distance between carbon atom in $CO_2$ and surface Pt atom, as well as hydrogen atom and surface Pt atom. **b** Similar PES for Pd (111) surface. **c** Absolute error (AE) in forward and backward activation barrier energy ($E_a$). Left two panels indicate results for Pt surface while right two panels show results for Pd surface.

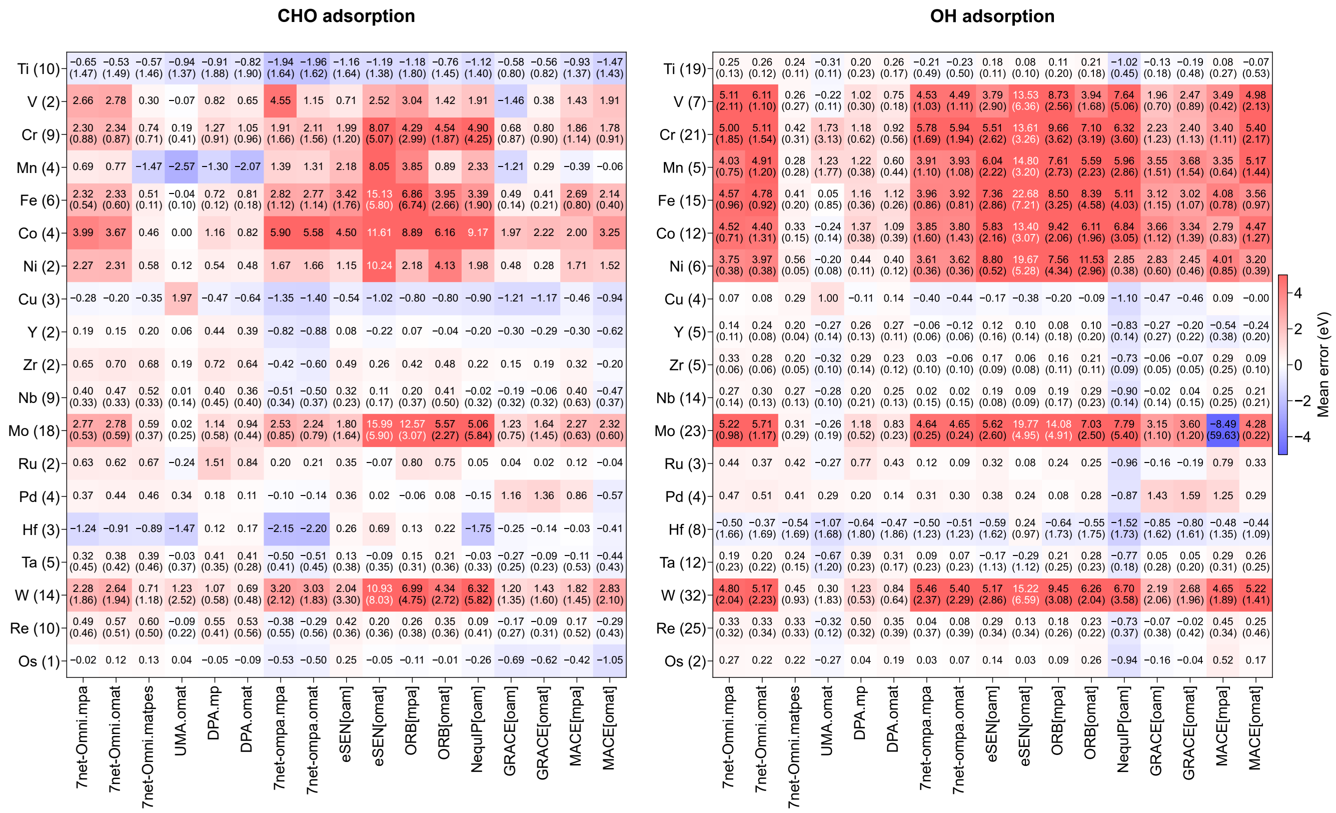


**Supplementary Figure 24**: **Adsorption on transition metal nitrides.** Heatmap of mean errors (eV) in adsorption energies for CHO (left) and OH (right) adsorption on transition metal nitrides, calculated using different uMLIPs. Each row corresponds to a transition metal element, where the total number of adsorption reactions for each metal is indicated in parentheses to the right of the element. Standard deviations are shown below the mean error values when the number of reactions exceeds four. The color and its intensity denotes the sign and magnitude of the mean error, respectively. Reference adsorption energies at the PBE level of theory and corresponding geometries are taken from ref. [1]. For each adsorbate–slab pair, the most stable configuration is selected. Most models show spurious overestimation of the adsorption energy for oxygen-containing adsorbates on nitrides of $U$-corrected transition metals, except for 7net-Omni.matpes, UMA, and DPA.

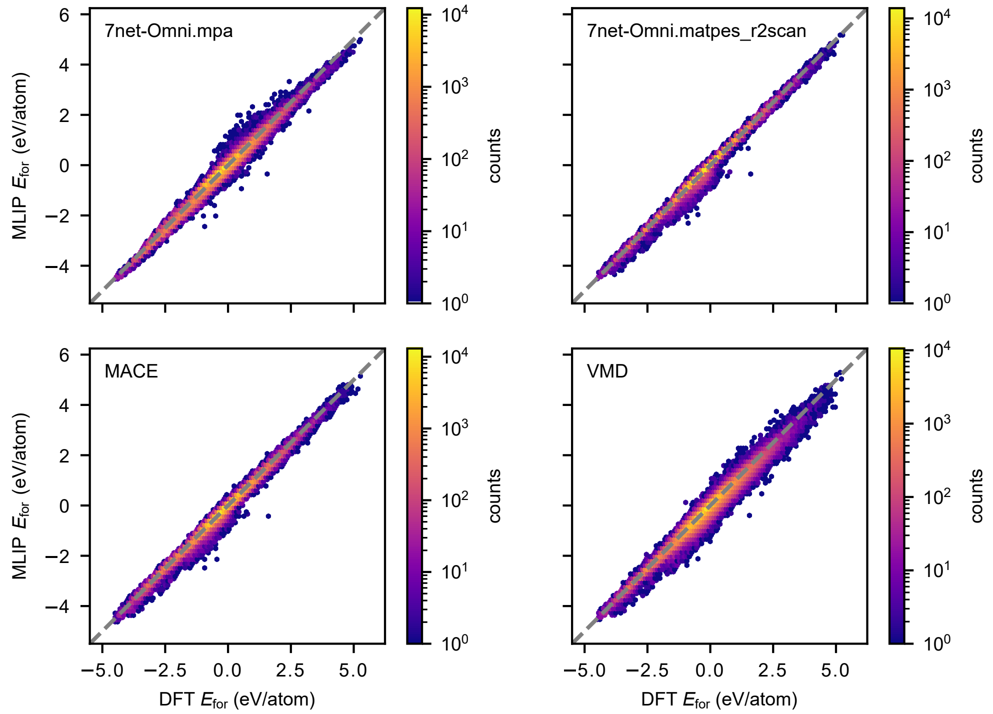


**Supplementary Figure 25**: **Party plots of formation energies of inorganic crystals.** Reference values are calculated with meta-GGA SCAN functional for the structures relaxed with PBEsol functional. Color at each region indicates the count of data points. To calculate formation energy from 7net-Omni.mpa, we utilized energy correction suggested in Ref. [2], which employs mixing scheme between GGA and GGA+$U$.

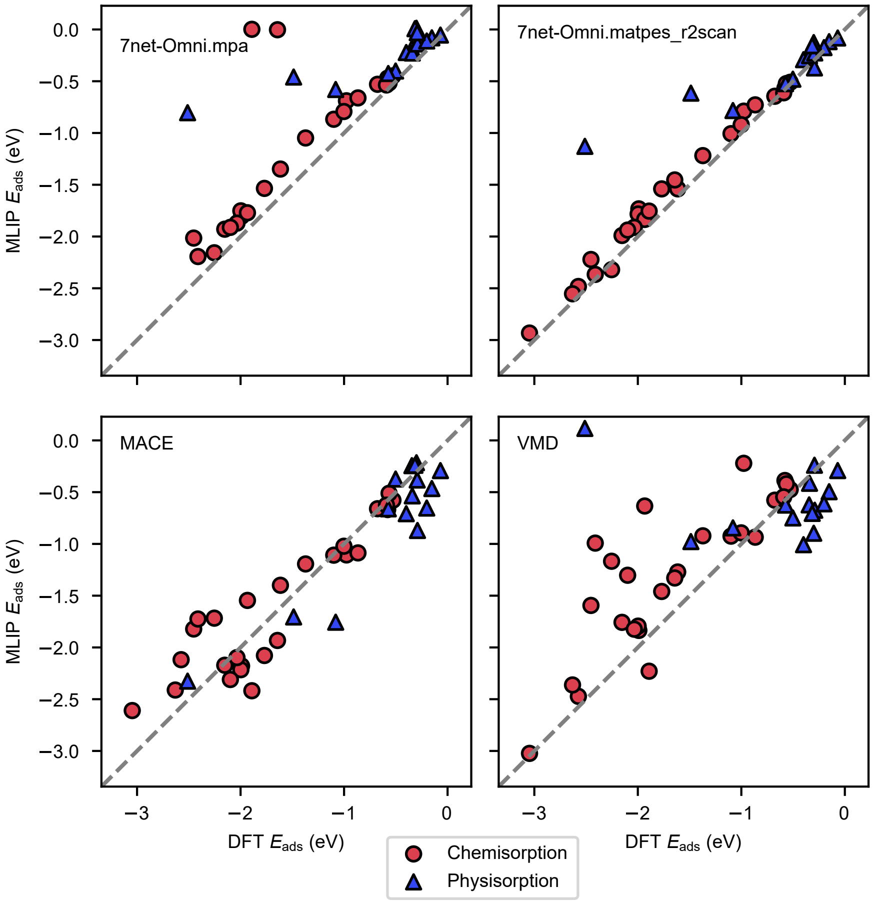


**Supplementary Figure 26**: **Party plots of adsorption energies in ADS41 benchmark.** Reference values are calculated with meta-GGA $r^2$SCAN functional. Circle and triangle markers indicate chemisorption and physisorption, respectively.

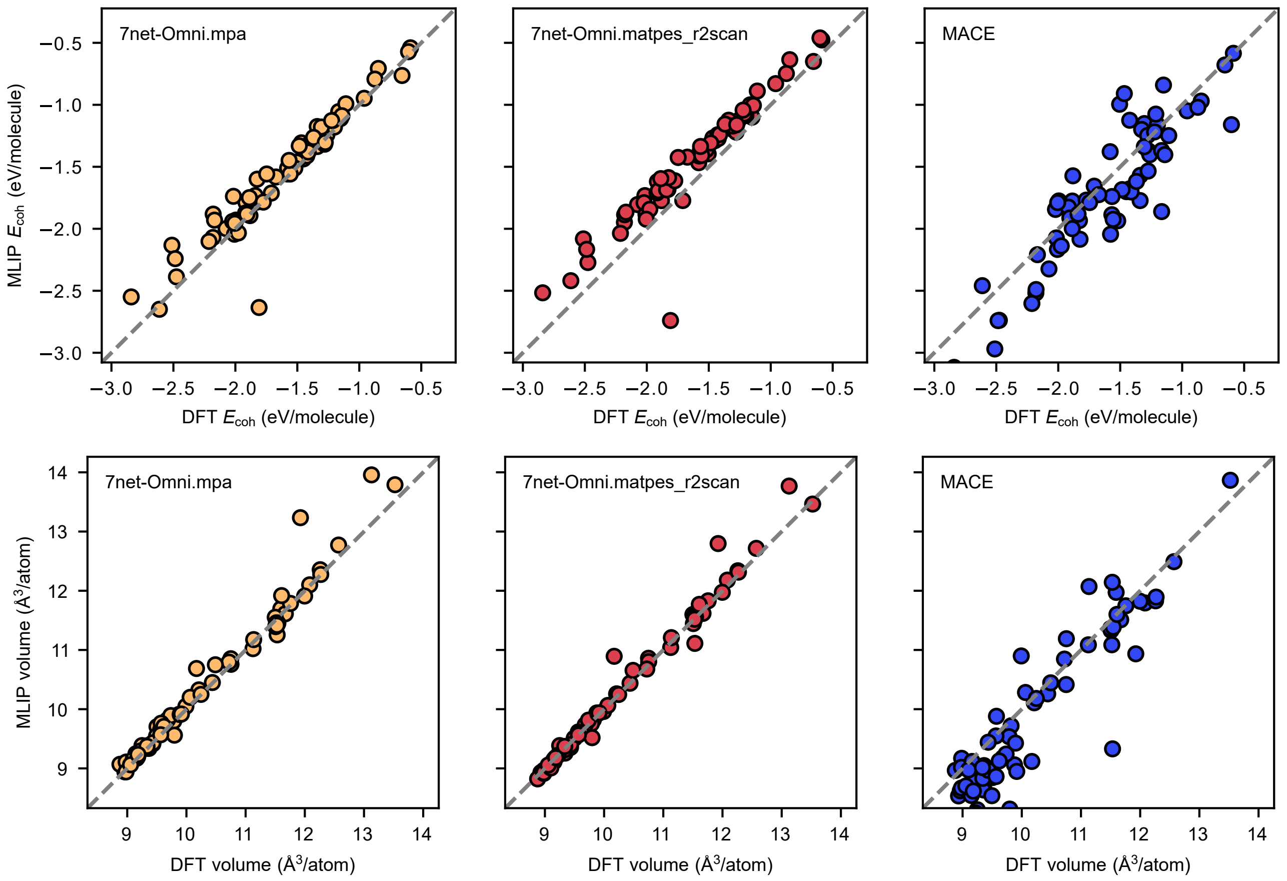


**Supplementary Figure 27**: **Party plots of cohesive energies and equilibrium volumes in BMCOS1 benchmark.** Reference values are calculated at the r$^2$SCAN-D3 level of theory. The first row illustrates results on cohesive energies and the second row depicts plots of equilibrium volume of molecular crystals.

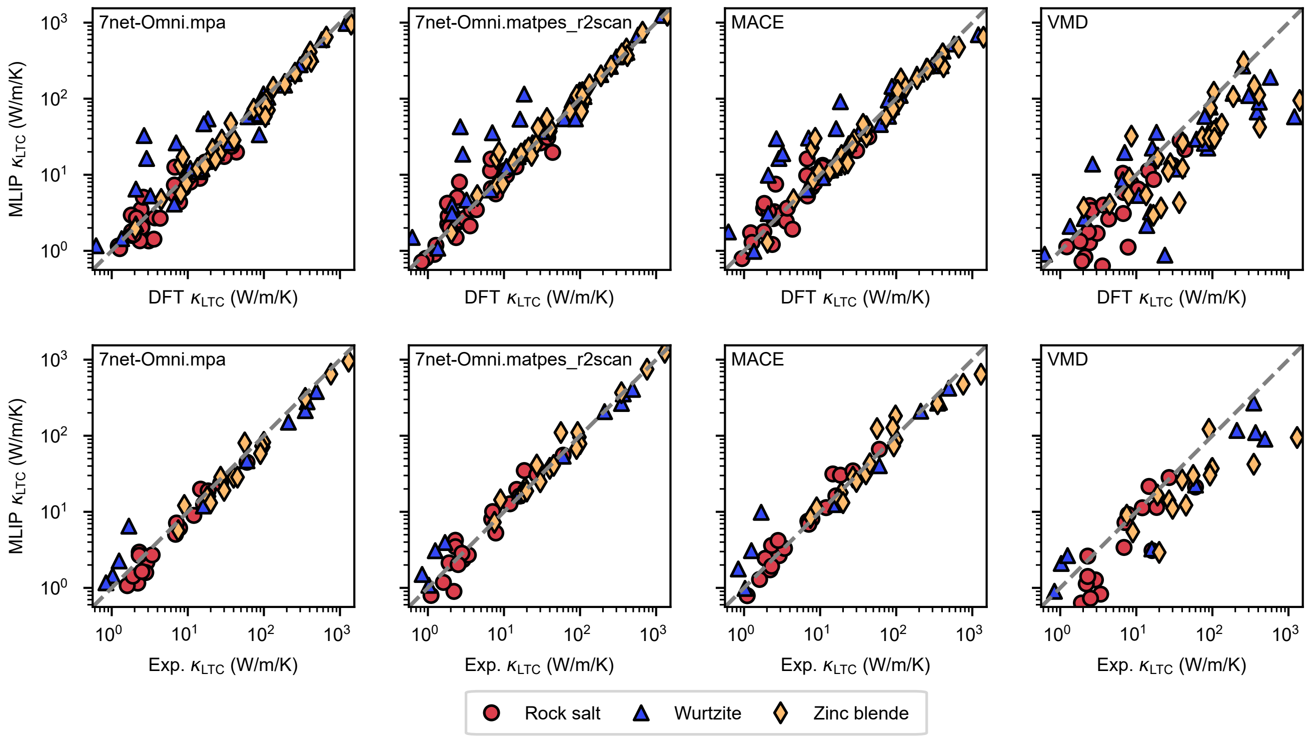


**Supplementary Figure 28**: **Party plots of lattice thermal conductivity ($\kappa_{\mathrm{LTC}}$) in binary solids.** The first row illustrates MLIP results compared to $\kappa_{\mathrm{LTC}}$ calculated by r$^2$SCAN functional while the second row depicts correlation compared with experimental $\kappa_{\mathrm{LTC}}$. Circle, triangle and diamond markers indicate prototype of corresponding materials (rock salt, wurtzite and zinc blende, respectively).

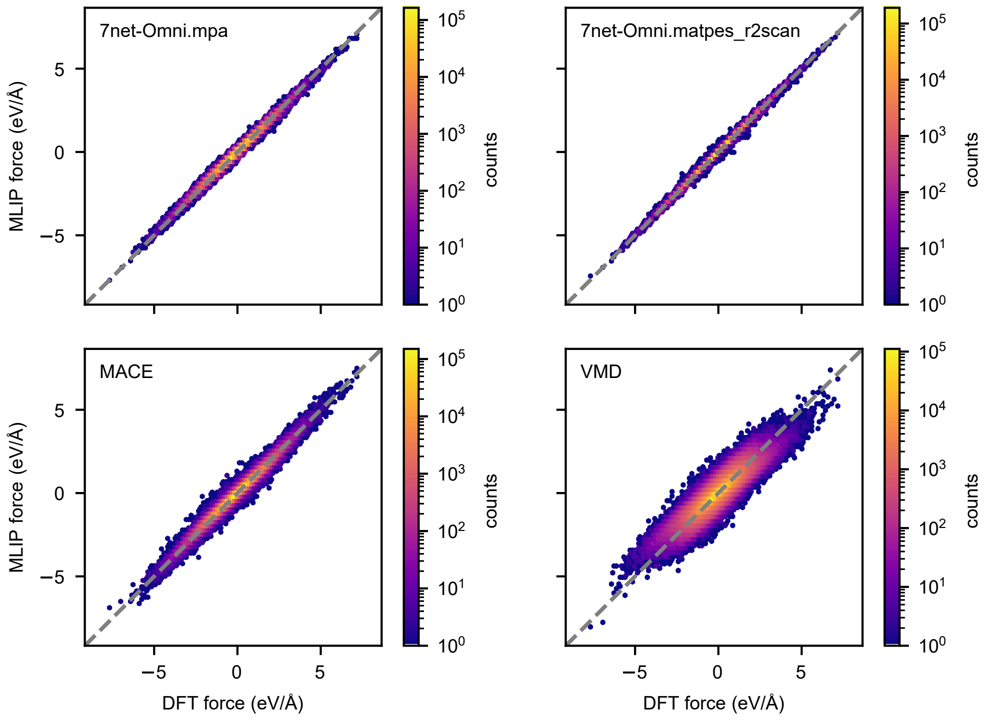


**Supplementary Figure 29**: **Party plots of force components obtained from ab initio molecular dynamics simulations of argyrodite $Li_6PS_5Cl$.** Molecular dynamics simulations are conducted using $r^2$SCAN functional. Color at each region indicates the count of data points.

# References


[1] Yohannes, A.G., Lee, C., Talebi, P., Mok, D.H., Karamad, M., Back, S., Siahrostami, S.: Combined High-Throughput DFT and ML Screening of Transition Metal Nitrides for Electrochemical $CO_2$ Reduction. ACS Catalysis **13**(13), 9007–9017 (2023)

[2] Jain, A., Hautier, G., Ong, S.P., Moore, C.J., Fischer, C.C., Persson, K.A., Ceder, G.: Formation enthalpies by mixing GGA and GGA+$U$ calculations. Phys. Rev. B **84**(4), 045115 (2011)
